# Supplementary material for: Interacting non-Hermitian edge and cluster bursts on a digital quantum processor
Source: arXiv:2503.14595 source file (2025-03-18)
Supplement: Supplementary file 1 [file supp.pdf]

# Interacting Non-Hermitian Edge and Cluster Bursts on a Digital Quantum Processor (Supplementary Information)

Jin Ming Koh,[1,2] Wen-Tan Xue,[3] Tommy Tai,[4] Dax Enshan Koh,[2,5,6] and Ching Hua Lee[3,*]

[1]*Department of Physics, Harvard University, Cambridge, Massachusetts 02138, USA*
[2]*Quantum Innovation Centre (Q.InC), Agency for Science, Technology and Research (A*STAR), 2 Fusionopolis Way, Innovis #08-03, Singapore 138634, Republic of Singapore*
[3]*Department of Physics, National University of Singapore, Singapore 117542, Republic of Singapore*
[4]*Department of Physics, Massachusetts Institute of Technology, Cambridge, Massachusetts 02142, USA*
[5]*Institute of High Performance Computing (IHPC), Agency for Science, Technology and Research (A*STAR), 1 Fusionopolis Way, #16-16 Connexis, Singapore 138632, Republic of Singapore*
[6]*Science, Mathematics and Technology Cluster, Singapore University of Technology and Design, 8 Somapah Road, Singapore 487372, Republic of Singapore*

## CONTENTS

List of Figures 1

List of Tables 2

1. Further details on model and time-dynamics 6
   A. Symmetries and equivalences of the quantum ladder Hamiltonian 6
   B. Speed limit on energy variation during non-Hermitian time-evolution 6

2. Further details on quantum simulation methods 8
   A. Implementation of uncontrolled and coherently controlled multi-qubit Pauli rotations 8
   B. Implementation of $\mathcal{M}_\mathrm{A}$ map and time steps 9
      a. An effective square root of $\mathcal{H}_\mathrm{A}$ is known or efficiently computable 9
      b. Circuit depth reduction by merging pairs of time steps 10
      c. Higher-order implementations of $\mathcal{M}_\mathrm{A}$ via many-term LCUs 11
      d. An effective square root of $\mathcal{H}_\mathrm{A}$ is not known 11

3. Further details on error suppression and mitigation methods 15
   A. Zero-noise extrapolation with physicality constraints 15
      a. Amplifying noise through local gate folding 16
      b. Randomizing coherent errors through Pauli twirling 16

4. Additional Results 17
   A. Additional experiment results on the canonical edge burst 17
   B. Spatially extended edge bursts with multiple interacting particles 20
   C. Alternative recovery of quantum state norm from algorithm success probability 22

References 23

## LIST OF FIGURES

S1 Detailed quantum simulation circuit structures and components . . . 14
S2 Canonical edge burst on $N = 8$ quantum ladder with different initial particle localization . . . 18
S3 Canonical edge burst on a smaller $N = 4$ quantum ladder . . . 19
S4 Additional results with two interacting particles . . . 20

* phylch@nus.edu.sg

S5 Spatially extended and ordered edge bursts with three interacting particles . . . . . . 21
S6 Comparison between quantum state norm recovery methods . . . . . . 22

## LIST OF TABLES

S1 Pauli decompositions of $\mathcal{H}_0^{\mathrm{eb}}$ Hamiltonian . . . . . . 3
S2 Hamiltonian $\mathcal{H}^{\mathrm{eb}}$ parameter values used in experiments and other specifications . . . . . . 3
S3 Superconducting quantum devices used in experiments. . . . . . . 4
S4 Performance characteristics of quantum devices used in experiments . . . . . . 4
S5 Operator pairs $P_1$ and $P_2$ used for Pauli twirling . . . . . . 5
S6 Higher-order linear combination of unitaries expansions for $\mathcal{M}_{\mathrm{A}}$. . . . . . . 11

$N = 4$

| Component | Pauli String | Coefficient |
|---|---|---|
| $\mathcal{H}_{\mathrm{H}}$ | IIX | $v_1$ |
| | IXX | $v_2/2$ |
| | IYZ | $v_2/2$ |
| | XXX | $v_2/4$ |
| | XYZ | $-v_2/4$ |
| | YXZ | $v_2/4$ |
| | YYX | $v_2/4$ |
| $\mathcal{H}_{\mathrm{A}}$ | III | $\gamma/2$ |
| | IIZ | $-\gamma/2$ |

$N = 8$

| Component | Pauli String | Coefficient |
|---|---|---|
| $\mathcal{H}_{\mathrm{H}}$ | IIIX | $v_1$ |
| | IIXX | $v_2/2$ |
| | IIYZ | $v_2/2$ |
| | IXXX | $v_2/4$ |
| | IXYZ | $-v_2/4$ |
| | IYXZ | $v_2/4$ |
| | IYYX | $v_2/4$ |
| | XXXX | $v_2/8$ |
| | XXYZ | $-v_2/8$ |
| | XYXZ | $-v_2/8$ |
| | XYYX | $-v_2/8$ |
| | YXXZ | $v_2/8$ |
| | YXYX | $v_2/8$ |
| | YYXX | $v_2/8$ |
| | YYYZ | $-v_2/8$ |
| $\mathcal{H}_{\mathrm{A}}$ | IIII | $\gamma/2$ |
| | IIIZ | $-\gamma/2$ |

Supplementary Table S1. Explicit Pauli decompositions of $\mathcal{H}_0^{\mathrm{eb}}$ Hamiltonian in the single-particle ($p = 1$) sector at $N = 4$ and $N = 8$ unit cells, given for illustration. Above $v_1$, $v_2$ are tight-binding hopping coefficients and $\gamma$ is an on-site loss rate—see Eq. (1) of main text or Eq. (7) of Methods. The general forms of Pauli decompositions of $\mathcal{H}_{\mathrm{H}}$ and $\mathcal{H}_{\mathrm{A}}$ components are written in Eq. (13) of Methods and used consistently thereafter in the description of our algorithms.

| Experiment | $N$ | $p$ | Regime | $v_1$ | $v_2$ | $\gamma$ | $U_r$ | Init. Locs. $\{x_0\}$ |
|---|---|---|---|---|---|---|---|---|
| Supplementary Figure S3a–S3d | 4 | 1 | Edge burst | 0.4 | 0.5 | 0.5 | - | $\{3\}$ |
| Supplementary Figure S3e | 4 | 1 | Trivial | 1 | 0.5 | 0.5 | - | $\{3\}$ |
| Main Figure 2a–d | 8 | 1 | Edge burst | 0.4 | 0.5 | 0.5 | - | $\{6\}$ |
| Main Figure 2e | 8 | 1 | Trivial | 1 | 0.5 | 0.5 | - | $\{6\}$ |
| Supplementary Figure S2a–S2d | 8 | 1 | Edge burst | 0.4 | 0.5 | 0.5 | - | $\{4\}$ |
| Supplementary Figure S2e | 8 | 1 | Edge burst | 1 | 0.5 | 0.5 | - | $\{4\}$ |
| Main Figure 3a, 3c | 64 | 1 | Edge burst | 0.4 | 0.5 | 1 | - | $\{51\}$ |
| Main Figure 3b, 3c | 64 | 1 | Trivial | 1 | 0.5 | 1 | - | $\{51\}$ |
| Main Figure 4b | 16 | 1 | Variable | $[0, 1]$ | 0.5 | 0.5 | - | $\beta = 0$ Gibbs |
| Main Figure 5a | 12 | 2 | Edge burst* | 0.4 | 0.5 | 1 | $U_r = 3\,\forall\, r \in [1]$ | $\{10, 12\}$ |
| Main Figure 5b | 12 | 2 | Trivial | 0.7 | 0.5 | 1 | $U_r = 3\,\forall\, r \in [1]$ | $\{10, 12\}$ |
| Main Figure 5c, Supplementary Figure S6a | 14 | 2 | Edge burst* | 0.4 | 0.5 | 1 | $U_r = 3\,\forall\, r \in [3]$ | $\{11, 14\}$ |
| Supplementary Figure S4a, S6b | 14 | 2 | Trivial* | 0.7 | 0.5 | 1 | $U_r = 3\,\forall\, r \in [3]$ | $\{11, 14\}$ |
| Main Figure 5d | 14 | 2 | Edge burst* | 0.4 | 0.5 | 1 | $U_r = 3\,\forall\, r \in [5]$ | $\{10, 14\}$ |
| Supplementary Figure S4b | 14 | 2 | Trivial* | 0.7 | 0.5 | 1 | $U_r = 3\,\forall\, r \in [5]$ | $\{10, 14\}$ |
| Main Figure 6a | 14 | 2 | Edge burst* | 0.4 | 0.5 | 1 | $U_r = 2\,\forall\, r \in [1]$ | $\{8, 9\}$ |
| Main Figure 6b | 14 | 2 | Trivial* | 0.7 | 0.5 | 1 | $U_r = 2\,\forall\, r \in [1]$ | $\{8, 9\}$ |
| Main Figure 6c | 14 | 2 | Edge burst* | 0.4 | 0.5 | 1 | $U_r = 2\,\forall\, r \in [3]$ | $\{8, 9\}$ |
| Main Figure 6d | 14 | 2 | Trivial* | 0.7 | 0.5 | 1 | $U_r = 2\,\forall\, r \in [3]$ | $\{8, 9\}$ |
| Supplementary Figure S5a | 13 | 3 | Edge burst* | 0.375 | 0.5 | 1 | $U_r = 5\,\forall\, r \in [1]$ | $\{9, 11, 13\}$ |
| Supplementary Figure S5b | 13 | 3 | Trivial* | 0.6 | 0.5 | 1 | $U_r = 5\,\forall\, r \in [1]$ | $\{9, 11, 13\}$ |
| Supplementary Figure S5c | 17 | 3 | Edge burst* | 0.375 | 0.5 | 1 | $U_r = 5\,\forall\, r \in [3]$ | $\{11, 14, 17\}$ |
| Supplementary Figure S5d | 17 | 3 | Trivial* | 0.6 | 0.5 | 1 | $U_r = 5\,\forall\, r \in [3]$ | $\{11, 14, 17\}$ |
| Supplementary Figure S5e | 20 | 3 | Edge burst* | 0.375 | 0.5 | 1 | $U_r = 5\,\forall\, r \in [5]$ | $\{12, 16, 20\}$ |
| Supplementary Figure S5f | 20 | 3 | Trivial* | 0.6 | 0.5 | 1 | $U_r = 5\,\forall\, r \in [5]$ | $\{12, 16, 20\}$ |

Supplementary Table S2. Values of hopping coefficients $v_1, v_2$, on-site loss rate $\gamma$, and interaction amplitudes $U_r$ parametrizing the non-Hermitian Hamiltonian $\mathcal{H}^{\mathrm{eb}}$ used in experiments. Also listed are the number of unit cells $N$ (the number of sites on the ladder is accordingly $2N$), number of bosons $p$, and initial boson localization used in the experiments. For ease of interpretation we label regimes canonically supporting the non-Hermitian edge burst as "Edge burst" ($v_1/v_2 \leq 1$) and regimes that do not as "Trivial" ($v_1/v_2 > 1$). The * mark denotes that the experiment involves multiple interacting bosons and is beyond the canonical setting of the non-Hermitian edge burst (*i.e.* single-particle non-interacting).

| Experiment | Devices Used |
|---|---|
| Supplementary Figure S3 | *ibm_hanoi* |
| Main Figure 2a–e, Supplementary Figure S2 | *ibm_hanoi*, *ibmq_mumbai* |
| Main Figure 3a–c | *ibm_sherbrooke*, *ibm_osaka*, *ibm_kyoto* |
| Main Figure 4b | *ibm_hanoi*, *ibmq_mumbai*, *ibm_osaka* |
| Main Figure 5a–d, Supplementary Figure S4, S6 | *ibm_osaka*, *ibm_kyoto*, *ibm_nazca* |
| Main Figure 6a–d | *ibm_torino*, *ibm_osaka*, *ibm_kyoto*, *ibm_nazca* |
| Supplementary Figure S5 | *ibm_sherbrooke*, *ibm_osaka*, *ibm_kyoto*, *ibm_nazca* |

Supplementary Table S3. Superconducting quantum devices used in experiments.

| Device | Qubits | 2Q Gate | 1Q Gate Error ($\times 10^{-4}$) | | | 2Q Gate Error ($\times 10^{-3}$) | | | Readout Error ($\times 10^{-2}$) | | |
|---|---|---|---|---|---|---|---|---|---|---|---|
| | | | 10% | 90% | Med. | 10% | 90% | Med. | 10% | 90% | Med. |
| *ibm_torino* | 133 | CZ | 1.77 | 9.50 | 3.06 | 2.44 | 13.5 | 4.62 | 0.89 | 5.84 | 2.01 |
| *ibm_sherbrooke* | 127 | ECR | 1.39 | 6.24 | 2.25 | 4.55 | 15.0 | 7.42 | 0.51 | 5.01 | 1.15 |
| *ibm_osaka* | 127 | ECR | 1.23 | 12.5 | 2.41 | 4.03 | 19.3 | 7.15 | 0.65 | 8.94 | 1.99 |
| *ibm_kyoto* | 127 | ECR | 1.46 | 10.5 | 2.68 | 4.56 | 19.4 | 8.01 | 0.61 | 8.15 | 1.51 |
| *ibm_nazca* | 127 | ECR | 1.90 | 8.74 | 3.15 | 6.00 | 24.2 | 10.7 | 0.87 | 7.65 | 2.67 |
| *ibm_hanoi* | 27 | CX | 1.55 | 6.02 | 2.18 | 4.40 | 16.1 | 7.60 | 0.67 | 3.19 | 1.09 |
| *ibmq_mumbai* | 27 | CX | 1.58 | 3.75 | 2.08 | 5.66 | 11.5 | 7.52 | 1.24 | 5.87 | 1.70 |

| Device | 1Q Gate Time (ns) | Readout Time (ns) | 2Q Gate Times (ns) | | | $T_1$ (μs) | | | $T_2$ (μs) | | |
|---|---|---|---|---|---|---|---|---|---|---|---|
| | | | 10% | 90% | Med. | 10% | 90% | Med. | 10% | 90% | Med. |
| *ibm_torino* | | 1560 | 84.0 | 124 | 84.0 | 62.3 | 250 | 171 | 42.5 | 220 | 125 |
| *ibm_sherbrooke* | 56.9 | 1244 | 533 | 533 | 533 | 157 | 379 | 273 | 48.7 | 321 | 183 |
| *ibm_osaka* | 60.0 | 1400 | 660 | 660 | 660 | 127 | 396 | 275 | 19.8 | 322 | 151 |
| *ibm_kyoto* | 60.0 | 1400 | 660 | 660 | 660 | 124 | 320 | 223 | 28.2 | 237 | 115 |
| *ibm_nazca* | 60.0 | 4000 | 660 | 660 | 660 | 115 | 286 | 194 | 32.8 | 239 | 136 |
| *ibm_hanoi* | 32.0 | 818 | 242 | 576 | 348 | 68.8 | 194 | 142 | 25.1 | 284 | 132 |
| *ibmq_mumbai* | 35.6 | 3513 | 277 | 640 | 405 | 54.6 | 130 | 108 | 58.4 | 251 | 149 |

Supplementary Table S4. Performance characteristics of quantum devices used in experiments. For quantities that vary between qubits on the same device, we provide $10^{\text{th}}$ and $90^{\text{th}}$ percentile and median values evaluated over all qubits on the device. Characteristics summarized here are based on routine (∼daily) calibration data of the machines, retrieved over a duration of four weeks in the middle of experiments.

| $P_1$ | $P_2$ |
|---|---|
| II | II |
| IX | IX |
| IY | ZY |
| IZ | ZZ |
| XI | XX |
| XX | XI |
| XY | YZ |
| XZ | YY |
| YI | YX |
| YX | YI |
| YY | XZ |
| YZ | XY |
| ZI | ZI |
| ZX | ZX |
| ZY | IY |
| ZZ | IZ |

Supplementary Table S5. List of operator pairs $P_1$ and $P_2$ used for Pauli twirling. Each CX gate in an experiment circuit to be twirled is replaced by $P_1(\mathrm{CX})P_2$ for $(P_1, P_2)$ randomly drawn from the list above, such that the action of the twirled CX remains invariant. See Methods for methodological details.

## Supplementary Note 1: Further details on model and time-dynamics

### A. Symmetries and equivalences of the quantum ladder Hamiltonian

The quantum ladder model examined in our study, which we described in Eqs. (1)–(2) of the main text and Eq. (7) of Methods, possesses a U(1) number-conserving symmetry in the hardcore boson species. Explicitly, the Hamiltonian $\mathcal{H}^{\text{eb}}$ is invariant under the rotation $c_{x\ell} \to e^{i\phi} c_{x\ell}$ and $c^\dagger_{x\ell} \to e^{-i\phi} c^\dagger_{x\ell}$ for any $\phi \in \mathbb{R}$ across all unit cells $x \in [1, N]$ and sublattice $\ell \in \{a, b\}$ on the ladder. This implies that the total particle number is a conserved quantity under time-evolution (*i.e.* is a constant of motion). This number conservation is discussed and made use of in numerous places, for example as a physical constraint for error mitigation, as described in the main text and Methods.

The non-interacting $\mathcal{H}_0^{\text{eb}}$ possesses additional symmetries that constrain its complex spectrum. Here, it is most convenient to consider the Bloch Hamiltonian without the imaginary loss term, $\overline{\mathcal{H}}_0^{\text{eb}}(k) = \mathcal{H}_0^{\text{eb}}(k) + i\gamma\mathbb{I}/2$, where the Bloch Hamiltonian $\mathcal{H}_0^{\text{eb}}(k)$ was given in Eq. (1) of the main text. Then we note the following symmetries,

- Chiral symmetry characterized by $\tau^y \overline{\mathcal{H}}_0^{\text{eb}}(k)\tau^y = -\overline{\mathcal{H}}_0^{\text{eb}}(k)$, which implies that the spectrum of $\overline{\mathcal{H}}_0^{\text{eb}}$ is inversion-symmetric, that is, eigenenergies come in pairs $(+E, -E)$.
- Time-reversal symmetry characterized by $\tau^x \overline{\mathcal{H}}_0^{\text{eb}}(-k)\tau^x = -\overline{\mathcal{H}}_0^{\text{eb}}(k)^\dagger$, which implies that the spectrum of $\overline{\mathcal{H}}_0^{\text{eb}}$ is reflection-symmetric about the real axis, that is, eigenenergies come in pairs $(E, E^*)$.

Above, $\tau^x, \tau^y, \tau^z$ are Pauli operators acting in the sublattice pseudospin space. Together, these constrain the complex spectrum of $\mathcal{H}_0^{\text{eb}}$ to be reflection-symmetric about both the $\text{Re}(E) = 0$ and $\text{Im}(E) = -\gamma/2$ lines, as observed in Figures 4b–c of the main text.

Lastly, as mentioned in the main text, the non-interacting quantum ladder model $\mathcal{H}_0^{\text{eb}}$ is unitarily equivalent to the non-Hermitian Su–Schrieffer–Heeger (SSH) model [1, 2] with left-right asymmetric hoppings. Explicitly, the transformation $R^\dagger_{\text{SSH}} \mathcal{H}_0^{\text{eb}}(k) R_{\text{SSH}}$ with the unitary pseudospin rotation $R_{\text{SSH}} = e^{-i\pi\sigma^x/4}$ maps $\mathcal{H}_0^{\text{eb}}(k)$ onto the canonical non-Hermitian SSH model [3] with intercell hopping $v_2$ and asymmetric intracell hoppings $v_1 \pm \gamma/2$. This equivalence immediately establishes the presence of the non-Hermitian skin effect (NHSE) on the quantum ladder model. A non-unitary similarity transformation involving site-dependent rescaling can map the quantum ladder model onto the Hermitian SSH model [2].

### B. Speed limit on energy variation during non-Hermitian time-evolution

As mentioned in the discussion of Section II G of the main text, while a time-independent non-Hermitian Hamiltonian is not energy-conserving in the same sense as a time-independent (and therefore continuously time-translation symmetric) Hermitian Hamiltonian of a closed quantum system is, it can nonetheless be shown that energy variations during time-evolution under a time-independent non-Hermitian Hamiltonian are bounded by a fixed limit. This speed limit is determined by the magnitude (*i.e.* norm) of the anti-Hermitian part of the Hamiltonian, relative to the Hermitian part.

Concretely, consider an arbitrary non-Hermitian Hamiltonian $\mathcal{H} = \mathcal{H}_{\text{H}} - i\mathcal{H}_{\text{A}}$, where $\mathcal{H}_{\text{H}}$ and $-i\mathcal{H}_{\text{A}}$ are its Hermitian and anti-Hermitian parts respectively. Without loss of generality, the Hamiltonian can be rescaled such that $\|\mathcal{H}_{\text{H}}\|_2 = 1$, where here $\|\cdot\|_2$ denotes the spectral norm. Starting from an initial normalized quantum state $\omega_0$, the state after evolution by time $t$ is

$$\omega_t = e^{-i\mathcal{H}t}\omega_0 e^{+i\mathcal{H}^\dagger t}. \tag{S1.1}$$

We evaluate the speed of change of energy of the state,

$$\begin{aligned}
\left|\frac{\mathrm{d}}{\mathrm{d}t}E_t\right| = \left|\frac{\mathrm{d}}{\mathrm{d}t}\langle\mathcal{H}\rangle_{\omega_t}\right| = \left|\frac{\mathrm{d}}{\mathrm{d}t}\mathrm{tr}(\mathcal{H}\omega_t)\right| &= \left|\frac{\mathrm{d}}{\mathrm{d}t}\mathrm{tr}\Big(\mathcal{H}e^{-i\mathcal{H}t}\omega_0 e^{+i\mathcal{H}^\dagger t}\Big)\right| \\
&= \left|\mathrm{tr}\left[\mathcal{H}\left(\frac{\mathrm{d}}{\mathrm{d}t}e^{-i\mathcal{H}t}\right)\omega_0 e^{+i\mathcal{H}^\dagger t} + \mathcal{H}e^{-i\mathcal{H}t}\omega_0\left(\frac{\mathrm{d}}{\mathrm{d}t}e^{+i\mathcal{H}^\dagger t}\right)\right]\right| \\
&= \left|\mathrm{tr}\Big[\mathcal{H}\left(-i\mathcal{H}\right)e^{-i\mathcal{H}t}\omega_0 e^{+i\mathcal{H}^\dagger t} + \mathcal{H}e^{-i\mathcal{H}t}\omega_0\left(+i\mathcal{H}^\dagger\right)e^{+i\mathcal{H}^\dagger t}\Big]\right| \\
&= \left|\mathrm{tr}\big[\left(\mathcal{H}^\dagger - \mathcal{H}\right)\mathcal{H}\omega_t\big]\right| \\
&= 2|\mathrm{tr}(\mathcal{H}_{\text{A}}\mathcal{H}\omega_t)|,
\end{aligned} \tag{S1.2}$$

where we have used the cyclic property of the trace. Then, noting that $\omega_t$ is a quantum state and is positive semidefinite, Hölder's inequality for inner product spaces implies

$$\left|\frac{\mathrm{d}}{\mathrm{d}t}E_t\right| \leq 2\|\mathcal{H}_\mathrm{A}\mathcal{H}\|_2 \operatorname{tr}(\omega_t). \tag{S1.3}$$

Lastly, noting that the spectral norm is sub-multiplicative and using the triangle inequality, we have

$$\begin{aligned}\left|\frac{\mathrm{d}}{\mathrm{d}t}E_t\right| &\leq 2\|\mathcal{H}_\mathrm{A}\|_2\|\mathcal{H}\|_2 \operatorname{tr}(\omega_t) \\ &\leq 2\|\mathcal{H}_\mathrm{A}\|_2 \left(\|\mathcal{H}_\mathrm{H}\|_2 + \|\mathcal{H}_\mathrm{A}\|_2\right) \operatorname{tr}(\omega_t) \\ &\leq 2\|\mathcal{H}_\mathrm{A}\|_2 \left(1 + \|\mathcal{H}_\mathrm{A}\|_2\right) \operatorname{tr}(\omega_t),\end{aligned} \tag{S1.4}$$

which is the speed limit we alluded to. Observe that for Hermitian Hamiltonians, for which $\mathcal{H}_\mathrm{A} = 0$, this bound reproduces energy conservation,

$$\left|\frac{\mathrm{d}}{\mathrm{d}t}E_t\right| \leq 0 \Longrightarrow \frac{\mathrm{d}}{\mathrm{d}t}E_t = 0. \tag{S1.5}$$

In the analysis above, the energy of the state $E_t$ is defined with respect to $\omega_t$ with no further normalization considerations. However, in the non-Hermitian setting, state normalization is not generically preserved—*i.e.* $\operatorname{tr}(\omega_t) \neq \operatorname{tr}(\omega_0) = 1$. Then there is no physical reason to forbid scalar rescaling of quantum states as in conventional Hermitian systems, that is, one can envision mathematical transformations $\omega_t \mapsto \alpha\omega_t$ for any $\alpha > 0$ to be allowed. Manifestly $E_t$ and $(\mathrm{d}/\,\mathrm{d}t)E_t$ as analyzed above are not invariant to such rescalings. To enforce invariance, we may consider $E_t$ and $(\mathrm{d}/\,\mathrm{d}t)E_t$ normalized by the quantum state norm $\operatorname{tr}(\omega_t)$. Then we have the compact result

$$\frac{1}{\operatorname{tr}(\omega_t)}\left|\frac{\mathrm{d}}{\mathrm{d}t}E_t\right| \leq 2\|\mathcal{H}_\mathrm{A}\|_2 \left(1 + \|\mathcal{H}_\mathrm{A}\|_2\right). \tag{S1.6}$$

## Supplementary Note 2: Further details on quantum simulation methods

### A. Implementation of uncontrolled and coherently controlled multi-qubit Pauli rotations

An exponentiated Pauli string $e^{-i\theta\sigma}$ for a coefficient $\theta \in \mathbb{R}$ and Pauli string $\sigma$ acting on $n$ qubits, also referred to as a multi-qubit Pauli rotation, can be implemented on a quantum circuit with the following standard construction [4],

$$e^{-i\theta\sigma} = B^\dagger E^\dagger R_1^z(2\theta) E B, \qquad B = \bigotimes_{j=1}^{n} B_j, \qquad E^\dagger = \prod_{\substack{j=2 \\ \sigma_j \neq \mathbb{I}}}^{n} \mathrm{CX}_{j1}, \qquad B_j = \begin{cases} \mathbb{I} & \sigma_j \in \{\mathbb{I}, Z\} \\ H & \sigma_j = X \\ HS^\dagger & \sigma_j = Y, \end{cases} \tag{S2.1}$$

where we have written $\sigma = \otimes_{j=1}^n \sigma_j$ for single-qubit Pauli operators $\sigma_j \in \{\mathbb{I}, X, Y, Z\}$, and we assume the first and last Paulis are non-trivial, $\sigma_1 \neq \mathbb{I}$ and $\sigma_n \neq \mathbb{I}$, without loss of generality. Here $B$ is a layer of Clifford single-qubit rotations acting as a basis transformation, $E$ is an entangler that connects qubits in the support of the Pauli string, $\mathrm{CX}_{jj'}$ is a CX gate with control and target on qubits $j$ and $j'$ respectively, and $H$ and $S$ are the Hadamard and phase gates respectively. The $R^z$ rotation gate in the middle of the construction acts only on a single qubit. See Supplementary Figure S1a for a circuit diagram.

The structure of the entangler $E$ above requires numerous long-range CX gates. In particular, CX gates connecting the $n^{\text{th}}$ qubit and the first qubit are needed, amongst others. This is problematic on devices with effectively linear nearest-neighbor (LNN) qubit connectivity, where qubits are connected only to adjacent ones in a one-dimensional chain. While in principle a long-range CX can be decomposed into nearest-neighbor CXs through the insertion of SWAP gates, which exchange the states of neighboring qubits and in turn can be implemented with 3 nearest-neighbor CXs, or a bridge gate construction [5] (see Supplementary Figures S1c and S1e for circuit illustrations), these decompositions are hugely expensive in the circuit depth and gate counts incurred.

An alternative implementation of the entangler $E$ uses a ladder of CX gates that span qubits in the support $\Lambda(\sigma)$ of $\sigma$, and reduces both the number of non-nearest-neighbor CX gates and their average range:

$$E^\dagger = \prod_{j=2}^{|\Lambda(\sigma)|} \mathrm{CX}_{\Lambda(\sigma)_j \Lambda(\sigma)_{j-1}}, \qquad \Lambda(\sigma) = (j = 1, 2, \ldots, n \,:\, \sigma_j \neq \mathbb{I}), \tag{S2.2}$$

which is illustrated in Supplementary Figure S1b. This implementation requires non-nearest-neighbor CX gates only to connect across qubits not in the support of $\sigma$. It is thus advantageous to use this structure on LNN qubit connectivity topologies, as is the case in our experiments.

The controlled versions of the exponentiated Pauli string $e^{-i\theta\sigma}$ are written

$$\begin{aligned} \mathrm{C}\left[e^{-i\theta\sigma}\right] &= |0\rangle\langle 0| \otimes \mathbb{I} + |1\rangle\langle 1| \otimes e^{-i\theta\sigma}, \\ \overline{\mathrm{C}}\left[e^{-i\theta\sigma}\right] &= |1\rangle\langle 1| \otimes \mathbb{I} + |0\rangle\langle 0| \otimes e^{-i\theta\sigma} = (X \otimes \mathbb{I})\mathrm{C}\left[e^{-i\theta\sigma}\right](X \otimes \mathbb{I}), \end{aligned} \tag{S2.3}$$

where we have introduced an additional qubit to act as the control, and C and $\overline{\mathrm{C}}$ denote coherent control by the $|0\rangle$ and $|1\rangle$ states of the control quit respectively. That is, $\mathrm{C}[e^{i\theta\sigma}]$ acts as the identity and as $e^{-i\theta\sigma}$ on the $n$ system qubits when the control qubit is in the $|0\rangle$ and $|1\rangle$ states respectively. The $\overline{\mathrm{C}}[e^{-i\theta\sigma}]$ gate is identical to $\mathrm{C}[e^{-i\theta\sigma}]$ but with the control states flipped, and can be implemented as $\mathrm{C}[e^{-i\theta\sigma}]$ sandwiched by $X$ gates on the control qubit.

A straightforward but naïve circuit construction for $\mathrm{C}[e^{-i\theta\sigma}]$ follows by adding controls to every gate in the circuit for $e^{-i\theta\sigma}$ as written in Eqs. (S2.1) and (S2.2) above. This turns the single-qubit Clifford gates in the $B$ layers into controlled Cliffords, the CX gates in $E$ into Toffoli gates (double-controlled $X$ gates), and the single-qubit $R^z$ rotation into a controlled $R^z$ rotation. Using the CX ladder implementation in Eq. (S2.2), we have explicitly

$$\mathrm{C}\left[e^{i\theta\sigma}\right] = CB^\dagger\, CE^\dagger\, CR_1^z(2\theta)\, CE\, CB, \qquad CB = \bigotimes_{j=1}^{n} CB_j, \qquad CE^\dagger = \prod_{j=2}^{|\Lambda(\sigma)|} \mathrm{CCX}_{\Lambda(\sigma)_j \Lambda(\sigma)_{j-1}}, \tag{S2.4}$$

where $\mathrm{CCX}_{jj'} = \mathrm{C}[\mathrm{CX}_{jj'}]$ is the Toffoli gate with the control ancillary qubit and qubit $j$ as controls, and qubit $j'$ as the target. But this construction is stupendously expensive, as controlled gates are deep when decomposed into 1- and 2-qubit basis gates satisfying qubit connectivities. For example, a Toffoli gate decomposes into 6 CXs disregarding connectivity [4, 6]; satisfying connectivity further increases this overhead as gates have to be introduced to bridge between non-adjacent qubits.

A much more efficient construction for $\mathrm{C}[e^{-i\theta\sigma}]$ arises by noting that the circuits in Eqs. (S2.1) and (S2.2) are symmetric, $E^\dagger E = \mathbb{I}$ and $B^\dagger B = \mathbb{I}$, and so without the $R^z$ in the middle the circuit collapses into the identity. Then

$$\mathrm{C}\left[e^{i\theta\sigma}\right] = B^\dagger E^\dagger \, \mathrm{C}R_1^z(2\theta) \, EB \tag{S2.5}$$

and the $\mathrm{C}R^z$ gate decomposes compactly into a pair of CX gates and a pair of single-qubit $R^z$ rotations. See Supplementary Figures S1f and S1g for circuit diagrams. This construction for $\mathrm{C}\left[e^{-i\theta\sigma}\right]$ is only slightly more expensive than the uncontrolled $e^{-i\theta\sigma}$ itself, incurring a pair of CXs to connect to the control qubit and an additional single-qubit $R^z$ rotation. We use this implementation in our experiments.

### B. Implementation of $\mathcal{M}_\mathrm{A}$ map and time steps

We reproduce the defining requirement of the map $\mathcal{M}_\mathrm{A}$ as written in Eq. (12) of Methods here,

$$\mathcal{M}_\mathrm{A}(\rho) = \mathcal{N}\left[e^{-\mathcal{H}_\mathrm{A}\Delta t}\rho e^{-\mathcal{H}_\mathrm{A}\Delta t}\right] + \mathcal{O}\left(\frac{1}{m^2}\right), \tag{S2.6}$$

for a Hermitian Hamiltonian $\mathcal{H}_\mathrm{A}$, any arbitrary state $\rho$, and simulation time step $\Delta t = t/m$ for a number of time steps $m$. In the context of our present work, $\mathcal{H}_\mathrm{A}$ originates from a parent Hamiltonian $\mathcal{H} = \mathcal{H}_\mathrm{H} - i\mathcal{H}_\mathrm{A}$ which need not be Hermitian, where $\mathcal{H}_\mathrm{H}$ and $-i\mathcal{H}_\mathrm{A}$ are the Hermitian and anti-Hermitian components of the Hamiltonian respectively. As written above, the action of $\mathcal{M}_\mathrm{A}$ is to implement normalized imaginary time-evolution under $\mathcal{H}_\mathrm{A}$.

#### a. *An effective square root of $\mathcal{H}_\mathrm{A}$ is known or efficiently computable*

In the case that a Hermitian auxiliary Hamiltonian $\mathcal{R}$ is known or efficiently computable such that $\mathcal{R}^2 = \mathcal{H}_\mathrm{A}$, a linear combination of unitaries (LCU) construction implementing an action $W \propto U_+ + U_-$ with $U_\pm$ approximating forward and backward time-evolution by $\mathcal{R}$ can be used to realize the $\mathcal{M}_\mathrm{A}$ map, as described in Methods. That is, supposing that we have circuit components $U_\pm$ such that

$$U_\pm = e^{\pm i\mathcal{R}\sqrt{2\Delta t}} + \mathcal{O}(\Delta t^2), \tag{S2.7}$$

we can then assemble via LCU

$$\begin{aligned} W = \frac{1}{2}\left(U_+ + U_-\right) = \frac{1}{2}\left(e^{+i\mathcal{R}\sqrt{2\Delta t}} + e^{-i\mathcal{R}\sqrt{2\Delta t}} + \mathcal{O}(\Delta t^2)\right) &= 1 - \mathcal{R}^2\Delta t + \mathcal{O}(\Delta t^2) \\ &= e^{-\mathcal{H}_\mathrm{A}\Delta t} + \mathcal{O}(\Delta t^2), \end{aligned} \tag{S2.8}$$

and accordingly

$$\begin{aligned} \mathcal{M}_\mathrm{A}(\rho) = \mathcal{N}\left[W\rho W^\dagger\right] &= \mathcal{N}\left\{\left[e^{-\mathcal{H}_\mathrm{A}\Delta t} + \mathcal{O}(\Delta t^2)\right]\rho\left[e^{-\mathcal{H}_\mathrm{A}\Delta t} + \mathcal{O}(\Delta t^2)\right]\right\} \\ &= \mathcal{N}\left[e^{-\mathcal{H}_\mathrm{A}\Delta t}\rho e^{-\mathcal{H}_\mathrm{A}\Delta t}\right] + \mathcal{O}\left(\frac{1}{m^2}\right), \end{aligned} \tag{S2.9}$$

as desired. As introduced in Methods, the LCU construction implementing $W$ straightforwardly requires a single ancillary qubit prepared in the $|+\rangle$ state, which coherently controls $U_+$ and $U_-$ on the system register conditioned on its $|0\rangle$ and $|1\rangle$ states interchangeably, followed by a measurement in the $\sigma^x$-basis, equivalent to a Hadamard gate followed by a computational basis ($\sigma^z$-basis) measurement. The implementation succeeds when a $|0\rangle$-outcome is reported and fails otherwise. The ancillary qubit can be re-used through mid-circuit qubit reset before the next time step begins. Figure 1d in the main text illustrates the general LCU circuit structure, and Figures 1c and 1e illustrate the structure of time-evolution circuits assembled using this approach.

The square root $\mathcal{R}$ can be obtained from algebraic manipulation of $\mathcal{H}_\mathrm{A}$ in certain problems. Constraints on the symmetries and properties of the system can oftentimes also be exploited. There is broad literature on, for example, the roots of topological insulators and superconductors [7–10] and generalized classes of symmetry-protected topological or topologically ordered systems [11–16]. In situations where $\mathcal{R}$ is difficult to obtain, an alternative approach that requires only knowledge of $\mathcal{H}_\mathrm{A}$, albeit incurring higher overhead, can be used, which we detail in Supplementary Note 2 B d.

The coherently controlled forward and backward time-evolution blocks $U_+$ and $U_-$ in the LCU can be implemented by trotterization, as we mention in Methods. For this, we require the Pauli decomposition of $\mathcal{R}$, which then lends a standard implementation of $U_\pm$ through, for example, the first-order Trotter-Lie product formula,

$$\mathcal{R} = \sum_{k=1}^{K_\mathrm{R}} \gamma_k \eta^k, \qquad U_\pm = \prod_{k=1}^{K_\mathrm{R}} e^{\pm i\gamma_k \eta^k \sqrt{2\Delta t}}, \qquad \mathrm{C}U_\pm = \prod_{k=1}^{K_\mathrm{R}} \mathrm{C}\left[e^{\pm i\gamma_k \eta^k \sqrt{2\Delta t}}\right] \tag{S2.10}$$

where coefficients $\gamma_k \in \mathbb{R}$ and $\eta^k$ are Pauli strings. That is, the time-evolution circuits for $U_\pm$ comprise layers of multi-qubit Pauli rotations (*i.e.* exponentiated Pauli strings), and accordingly $\mathrm{C}U_\pm$ can be implemented as layers of coherently controlled multi-qubit Pauli rotations. We discussed in Supplementary Note 2 A the efficient implementation of controlled multi-qubit Pauli rotations at the gate level on hardware.

A relevant question concerns the conditions under which $\mathcal{R}$ exists. A positive semidefinite Hermitian $\mathcal{H}_\mathrm{A}$ always possesses a square root $\mathcal{R}$ that is positive semidefinite and Hermitian. In the case that $\mathcal{H}_\mathrm{A}$ is not positive semidefinite, one can trivially introduce an energy offset to make it so, $\mathcal{H}_\mathrm{A} \to \mathcal{H}_\mathrm{A} + \lambda\mathbb{I}$, for any $\lambda \geq |\lambda_\mathrm{min}|$ where $\lambda_\mathrm{min}$ is the smallest eigenenergy of $\mathcal{H}_\mathrm{A}$. Such an energy offset is inconsequential to the normalized time-evolution, as

$$\mathcal{N}\left[e^{-(\mathcal{H}_\mathrm{A}+\lambda\mathbb{I})\Delta t}\rho e^{-(\mathcal{H}_\mathrm{A}+\lambda\mathbb{I})\Delta t}\right] = \mathcal{N}\left[e^{-2\lambda\Delta t}e^{-\mathcal{H}_\mathrm{A}\Delta t}\rho e^{-\mathcal{H}_\mathrm{A}\Delta t}\right] = \mathcal{N}\left[e^{-\mathcal{H}_\mathrm{A}\Delta t}\rho e^{-\mathcal{H}_\mathrm{A}\Delta t}\right], \tag{S2.11}$$

and therefore works as a trick of convenience to realize well-defined choices of $\mathcal{R}$. Here, on grounds of physicality of the system of interest, we assume that the spectrum of $\mathcal{H}_\mathrm{A}$ is bounded from below, such that $\lambda_\mathrm{min}$ is finite. The minimum eigenenergy $\lambda_\mathrm{min}$ can be estimated from the algebraic structure of $\mathcal{H}_\mathrm{A}$ or numerically. Alternatively, without additional calculation, a simple conservative, but typically much excessive, choice is $\lambda = \sum_{k=1}^{K_\mathrm{A}} |\beta_k|$, where $\beta_k$ are the coefficients of the Pauli decomposition of $\mathcal{H}_\mathrm{A}$ as written in Eq. (13) of Methods.

In the present context of the edge burst, it was not necessary to invoke this energy shift as $\mathcal{H}_\mathrm{A}^\mathrm{eb}$ is positive semidefinite, as can be seen from Eq. (8) of Methods. In fact, by leveraging the on-site structure of $\mathcal{H}_\mathrm{A}^\mathrm{eb}$, we were able to obtain a Hermitian auxiliary Hamiltonian $\mathcal{H}_\mathrm{aux}^\mathrm{eb}$ taking the role of $\mathcal{R}$, such that the normalized superposition of its forward and backward time-evolutions via LCU implements the $e^{-\mathcal{H}_\mathrm{A}^\mathrm{eb}\Delta t}$ evolution of $\mathcal{M}_\mathrm{A}$ exactly, instead of to $\mathcal{O}(1/m^2)$ error as demanded generally here. We detailed this optimization in Methods. The implementation of the forward and backward time-evolutions via first-order trotterization, however, re-introduces $\mathcal{O}(1/m^2)$ approximation error, so the reduction in error from this optimization is sub-dominant. On general $\mathcal{H}_\mathrm{A}$ with complicated, possibly interacting, structure, we expect that such modifications to achieve errorless LCUs would be difficult; but we re-iterate that they are unnecessary for the simulation methodology to work.

### b. *Circuit depth reduction by merging pairs of time steps*

We remark that a general circuit optimization trick can be invoked for every pair of time steps, that roughly halves the circuit depth. We perform a re-ordering of $\mathcal{M}_\mathrm{H}$ and $\mathcal{M}_\mathrm{A}$ in the second time step,

$$(\mathcal{M}_\mathrm{A} \circ \mathcal{M}_\mathrm{H})^2(\rho) = (\mathcal{M}_\mathrm{H} \circ \mathcal{M}_\mathrm{A} \circ \mathcal{M}_\mathrm{A} \circ \mathcal{M}_\mathrm{H})(\rho) + \mathcal{O}\left(\frac{1}{m^2}\right), \tag{S2.12}$$

as the commutator of $\mathcal{M}_\mathrm{H}$ and $\mathcal{M}_\mathrm{A}$ acting on $\rho$ is of order $\mathcal{O}(\Delta t^2)$, and considering the middle consecutive $\mathcal{M}_\mathrm{A} \circ \mathcal{M}_\mathrm{A}$, one observes

$$\begin{aligned} W^2 \propto (U_+ + U_-)^2 &= \left(e^{+i\mathcal{R}\sqrt{2\Delta t}} + e^{-i\mathcal{R}\sqrt{2\Delta t}} + \mathcal{O}(\Delta t^2)\right)^2 \\ &= \left(\mathbb{I} + e^{-2i\mathcal{R}\sqrt{2\Delta t}} + \mathcal{O}(\Delta t^2)\right)\left(\mathbb{I} + e^{+2i\mathcal{R}\sqrt{2\Delta t}} + \mathcal{O}(\Delta t^2)\right), \end{aligned} \tag{S2.13}$$

which informs us that the same action across two time steps can be realized to the same $\mathcal{O}(1/m^2)$ error but restructured in the following way,

$$(\mathcal{M}_\mathrm{A} \circ \mathcal{M}_\mathrm{H})^2(\rho) = (\mathcal{M}_\mathrm{H} \circ \mathcal{M}_{\mathrm{A}-} \circ \mathcal{M}_{\mathrm{A}+} \circ \mathcal{M}_\mathrm{H})(\rho) + \mathcal{O}\left(\frac{1}{m^2}\right), \tag{S2.14}$$

where

$$\mathcal{M}_{\mathrm{A}\pm}(\rho) = \mathcal{N}\left[\left(\mathbb{I} + e^{\mp 2i\mathcal{R}\sqrt{2\Delta t}}\right)\rho\left(\mathbb{I} + e^{\pm 2i\mathcal{R}\sqrt{2\Delta t}}\right)\right] + \mathcal{O}\left(\frac{1}{m^2}\right). \tag{S2.15}$$

That is, the first map $\mathcal{M}_{A+}$ requires an LCU that superposes the unitaries $\mathbb{I}$ and forward time-evolution by $2\mathcal{R}$, and the second map $\mathcal{M}_{A-}$ requires an LCU that superposes the unitaries $\mathbb{I}$ and backward time-evolution by $2\mathcal{R}$. Now, we note that the implementation of the $\mathbb{I}$ unitary portions in the LCU is trivial, as a coherently controlled-$\mathbb{I}$ is simply the identity—*i.e.* no gates at all are required.

Therefore, this optimized implementation of $(\mathcal{M}_A \circ \mathcal{M}_A)^2$ requires only two controlled time-evolution unitaries (forward and backward by $2\mathcal{R}$), compared to the original four (two pairs of forward and backward by $\mathcal{R}$). We illustrate this circuit transformation in Supplementary Figures S1i and S1j. As the time-evolution unitaries are expensive and account for an overwhelming majority of the depth of the overall quantum simulation circuits, this optimization is hugely beneficial. We employed this technique in all of our experiments,

### *c. Higher-order implementations of $\mathcal{M}_A$ via many-term LCUs*

In the main text, Methods, and Supplementary Note 2 B a, we considered mainly an $\mathcal{M}_A$ that approximates normalized time-evolution by $-i\mathcal{H}_A$ to $\mathcal{O}(1/m^2)$ error, as that is sufficient for our quantum simulation methodology for non-Hermitian Hamiltonian as a whole to work. This defining requirement on $\mathcal{M}_A$ was written in Eq. (12) of Methods and repeated in Eq. (S2.6). But it can also be of interest to examine more advanced realizations of $\mathcal{M}_A$ that approximates the time-evolution to higher-order error,

$$\mathcal{M}_A(\rho) = \mathcal{N}\left[e^{-\mathcal{H}_A\Delta t}\rho e^{-\mathcal{H}_A\Delta t}\right] + \mathcal{O}\left(\frac{1}{m^\kappa}\right), \tag{S2.16}$$

for orders $\kappa \geq 2$. As described in Methods, in particular Eq. (15) and the surrounding discussion, the general strategy to obtain such realizations is to consider LCU expansions of the form

$$A_0\mathbb{I} + \sum_{b=1}^{B} A_b\left(e^{+i\mathcal{R}\Delta\tau_b} + e^{-i\mathcal{R}\Delta\tau_b}\right) = e^{-\mathcal{H}_A\Delta t} + \mathcal{O}\left(\frac{1}{m^\kappa}\right), \tag{S2.17}$$

for coefficients $A_0, \ldots, A_B \geq 0$ and rescaled simulation times $\{\Delta\tau_b\}_b$, and to match their Taylor expansions order-by-order on both sides. This leads to a system of polynomial equations that can then be solved. Generally, for any $\kappa \geq 2$, candidate LCU expansions realizing $\mathcal{M}_A$ can be found this way, and it is generally beneficial to select a solution with a minimal number of term pairs $B$ as this directly reduces circuit depth and the number of ancillary qubits needed to implement the LCU. We provide some examples of higher-order expansions with a minimal number of terms in Supplementary Table S6.

| $\kappa$ | Expansion | # Anc. Qubits |
|---|---|---|
| 2 | $e^{\pm iR\sqrt{2\Delta t}}$ | 1 |
| 3 | $4\mathbb{I} + e^{\pm iR\sqrt{6\Delta t}}$ | 2 |
| 4 | $(3-\sqrt{6})e^{\pm iR\sqrt{2(3+\sqrt{6})\Delta t}} + (3+\sqrt{6})e^{\pm iR\sqrt{2(3-\sqrt{6})\Delta t}}$ | 2 |
| 5 | $32\mathbb{I} + (7-2\sqrt{10})e^{\pm iR\sqrt{2(5+\sqrt{10})\Delta t}} + (7+2\sqrt{10})e^{\pm iR\sqrt{2(5-\sqrt{10})\Delta t}}$ | 3 |

Supplementary Table S6. Examples of linear combination of unitaries (LCU) expansions that approximate the non-unitary (imaginary) time-evolution propagator $e^{-\mathcal{H}_A\Delta t}$ for a Hermitian Hamiltonian $\mathcal{H}_A$ to $\mathcal{O}(1/m^\kappa)$ error, and thus can be used to implement the $\mathcal{M}_A$ map used in our time-evolution algorithm for general non-Hermitian Hamiltonians. The $\kappa = 2$ case corresponds to the setting discussed in the main text, Methods, and Supplementary Note 2 B a. Higher $\kappa$ beyond those presented here can be achieved by using more terms in the LCU expansions. Here $\mathcal{R}$ is any Hermitian Hamiltonian such that $\mathcal{R}^2 = \mathcal{H}_A$, we use the shorthand $e^{\pm iA} = e^{+iA} + e^{-iA}$, and we present the expansions up to overall normalization factors that are omitted.

### *d. An effective square root of $\mathcal{H}_A$ is not known*

In the case that a square root of $\mathcal{H}_A$ is not known or cannot be efficiently found, there is an alternative, more general approach of realizing $\mathcal{M}_A$, albeit requiring an extra ancillary qubit register in addition to the LCU ancillary qubit(s). Just like the LCU ancillary qubits, this ancillary qubit register can be re-used through mid-circuit qubit reset before the next time step.

Recall that by premise $\mathcal{H}$ is local and thus so is $\mathcal{H}_\mathrm{A}$; we assume they are $l$-local, that is, they comprise terms that act on at most $l \in \mathcal{O}(1)$ sites each on the system, independent of the system size. Then we can write

$$\mathcal{H}_\mathrm{A} = \sum_{k=1}^{L_\mathrm{A}} \kappa_k h_k, \tag{S2.18}$$

for real coefficients $\kappa_k > 0$ and Hermitian $h_k$ that each have support on at most $l$ sites, and a number of terms $L_\mathrm{A}$ that is polynomial in the system size. For simplicity, we assume $h_k$ are positive semidefinite; this can always be made the case by adding suitable energy offsets to $\mathcal{H}_\mathrm{A}$, whose spectrum we assume to be lower-bounded on grounds of physicality, or alternatively to each $h_k$, in a similar fashion as discussed in Supplementary Note 2 B a. Then there exist positive semidefinite Hermitian $r_k$ for each $h_k$ such that $r_k^2 = h_k$. Either these are algebraically known from the form of $h_k$, or they can be efficiently computed, since each $h_k$ acts only on $l$ sites and can each be efficiently processed.

Now we consider the larger Hermitian Hamiltonian

$$\mathcal{L} = \sum_{k=1}^{L_\mathrm{A}} \sqrt{\kappa_k} r_k \otimes \left( |k\rangle_\mathrm{a} \langle 0|_\mathrm{a} + |0\rangle_\mathrm{a} \langle k|_\mathrm{a} \right), \tag{S2.19}$$

where we have introduced an ancillary Hilbert space that is at least $(L_\mathrm{A}+1)$-dimensional, that is, comprising at least $\lceil \log_2(L_\mathrm{A}+1) \rceil$ qubits, labeled by the subscript 'a' above. As defined, $\mathcal{L}$ is Hermitian, and one observes

$$\mathcal{L}^{2p} \left( |\psi\rangle \otimes |0\rangle_\mathrm{a} \right) = \left[ (\mathcal{H}_\mathrm{A})^p |\psi\rangle \right] \otimes |0\rangle_\mathrm{a}, \tag{S2.20}$$

for any power $p \in \mathbb{N}$ and any system state $|\psi\rangle$. That is, given that the ancillary register starts in state $|0\rangle_\mathrm{a}$, the action of $\mathcal{L}^{2p}$ is identical to that of $(\mathcal{H}_\mathrm{A})^p$ on the system qubits. Note that the ancillary register is brought back to $|0\rangle_\mathrm{a}$ after being acted upon by $\mathcal{L}^{2p}$, and indeed is entirely disentangled with the system qubits.

In the same spirit as in Supplementary Note 2 B a, we consider an LCU construction implementing $\overline{W} \propto (\overline{U}_+ + \overline{U}_-)$ with $\overline{U}_\pm$ approximating forward and backward time-evolution by $\mathcal{L}$ to $\mathcal{O}\big(1/m^2\big)$ error. The difference is that $\overline{U}_\pm$ here act jointly on the system and ancillary qubit register, whereas $U_\pm$ before acted only on the system register with no involvement of any ancillae. Explicitly, supposing that we have circuit components $\overline{U}_\pm$ such that

$$\overline{U}_\pm = e^{\pm i \mathcal{L} \sqrt{2\Delta t}} + \mathcal{O}\big(\Delta t^2\big), \tag{S2.21}$$

we find

$$\begin{aligned} \overline{W} \left( |\psi\rangle \otimes |0\rangle_\mathrm{a} \right) = \frac{1}{2} \left( \overline{U}_+ + \overline{U}_- \right) \left( |\psi\rangle \otimes |0\rangle_\mathrm{a} \right) &= \frac{1}{2} \left( e^{+i\mathcal{L}\sqrt{2\Delta t}} + e^{-i\mathcal{L}\sqrt{2\Delta t}} + \mathcal{O}\big(\Delta t^2\big) \right) \left( |\psi\rangle \otimes |0\rangle_\mathrm{a} \right) \\ &= \left[ \mathbb{I} - \mathcal{L}^2 \Delta t + \mathcal{O}\big(\Delta t^2\big) \right] \left( |\psi\rangle \otimes |0\rangle_\mathrm{a} \right) \\ &= \left[ \left( \mathbb{I} - \mathcal{H}_\mathrm{A} \Delta t \right) |\psi\rangle \right] \otimes |0\rangle_\mathrm{a} + \mathcal{O}\big(\Delta t^2\big) \\ &= e^{-\mathcal{H}_\mathrm{A}\Delta t} |\psi\rangle \otimes |0\rangle_\mathrm{a} + \mathcal{O}\big(\Delta t^2\big). \end{aligned} \tag{S2.22}$$

Examining the system qubits, we find accordingly that

$$\begin{aligned} \mathcal{M}_\mathrm{A}(\rho) \equiv \mathcal{N} \left\{ \mathrm{tr}_\mathrm{a} \left[ \overline{W} \left( \rho \otimes |0\rangle_\mathrm{a} \langle 0|_\mathrm{a} \right) \overline{W}^\dagger \right] \right\} &= \mathcal{N} \left[ e^{-\mathcal{H}_\mathrm{A}\Delta t} \rho e^{-\mathcal{H}_\mathrm{A}\Delta t} \otimes |0\rangle_\mathrm{a} \langle 0|_\mathrm{a} \right] + \mathcal{O}\left( \frac{1}{m^2} \right) \\ &= \mathcal{N} \left[ e^{-\mathcal{H}_\mathrm{A}\Delta t} \rho e^{-\mathcal{H}_\mathrm{A}\Delta t} \right] + \mathcal{O}\left( \frac{1}{m^2} \right), \end{aligned} \tag{S2.23}$$

as desired. That is, an LCU construction implementing $\overline{W} \propto (\overline{U}_+ + \overline{U}_-)$ achieves $\mathcal{M}_\mathrm{A}$.

A remaining detail is how the coherently controlled $\overline{U}_\pm$ necessary in the LCU can be implemented. Without loss of generality we can perform processing (*i.e.* perform Pauli-basis decomposition) such that the $\{r_k\}_k$ terms in Eq. (S2.19) are Pauli strings. Likewise, we consider expressing the ancillary portion of each of the terms in $\mathcal{L}$ as Pauli strings. The details of this ancillary Pauli decomposition depends on the mapping chosen between the $(L_\mathrm{A}+1)$-dimensional Hilbert space considered here and a register of qubits—we discuss this below. The number of terms $L_\mathrm{A}$ in the Hamiltonian $\mathcal{L}$ remains polynomial in the system size after this rewriting. Ultimately, once $\mathcal{L}$ has been expressed entirely as Pauli strings, conventional trotterization, such as the first-order Trotter-Lie product formula, can be used to implement forward and backward time-evolution ($\overline{U}_\pm$) by $\mathcal{L}$ to error $\mathcal{O}\big(1/m^2\big)$ or better, in the same fashion as for $\mathcal{H}_\mathrm{A}$ originally discussed in the main text, Methods, and Supplementary Note 2 B a. Coherently controlling $\overline{U}_\pm$ entails adding controls to the Pauli rotations in the trotterization, and we have discussed an efficient implementation of these operations in Supplementary Note 2 A.

Lastly, we revisit the issue of mapping the ancillary space onto qubits. We discuss two natural choices:

- Using the minimum possible $\lceil \log_2(L_{\rm A}+1) \rceil$ number of ancillary qubits. Then the states $\{|k\rangle_{\rm a}\}_k$ can be mapped to the basis states of the ancillary qubits in, for example, binary ascending order,

$$|0\rangle_{\rm a} \equiv |0\ldots 00\rangle\,, \qquad |1\rangle_{\rm a} \equiv |0\ldots 01\rangle\,, \qquad |2\rangle_{\rm a} \equiv |0\ldots 10\rangle\,, \qquad |3\rangle_{\rm a} \equiv |0\ldots 11\rangle\,, \qquad \ldots. \tag{S2.24}$$

  While this is space-efficient (in terms of qubit count), an issue is that $|k\rangle_{\rm a}\langle 0|_{\rm a} + |0\rangle_{\rm a}\langle k|_{\rm a}$ can be relatively complicated when expressed in the Pauli basis of the qubits, containing a number of Pauli strings polynomial in $L_{\rm A}$ with weight up to $\lceil \log_2(L_{\rm A}+1) \rceil$. Therefore the circuit depth may not be particularly shallow.

- Choosing to use $L_{\rm A}$ qubits instead, we enjoy a reduction in circuit depth and complexity, at the expense of using a larger number of ancillary qubits. Here we map the states $\{|k\rangle_{\rm a}\}_k$ to the basis states of the ancillary qubits via one-hot encoding, for example,

$$|0\rangle_{\rm a} \equiv |000\ldots 0\rangle\,, \qquad |1\rangle_{\rm a} \equiv |100\ldots 0\rangle\,, \qquad |2\rangle_{\rm a} \equiv |010\ldots 0\rangle\,, \qquad |3\rangle_{\rm a} \equiv |001\ldots 0\rangle\,, \qquad \ldots. \tag{S2.25}$$

  That is, $\{|k\rangle_{\rm a}\}_k$ for $k > 0$ is identified with the ancillary qubit state where the $k^{\rm th}$ qubit is in $|1\rangle$ while all other qubits are in $|0\rangle$. Then straightforwardly,

$$|k\rangle_{\rm a}\langle 0|_{\rm a} + |0\rangle_{\rm a}\langle k|_{\rm a} \equiv \sigma^x_k, \tag{S2.26}$$

  within the subspace of qubit states associated with $\{|k\rangle_{\rm a}\}_k$, where $\sigma^x_k$ denotes the single-qubit $\sigma^x$ Pauli operator acting on the $k^{\rm th}$ ancillary qubit. Thus each $|k\rangle_{\rm a}\langle 0|_{\rm a} + |0\rangle_{\rm a}\langle k|_{\rm a}$ term maps to only a single-qubit Pauli operator. This is particularly simple to implement.

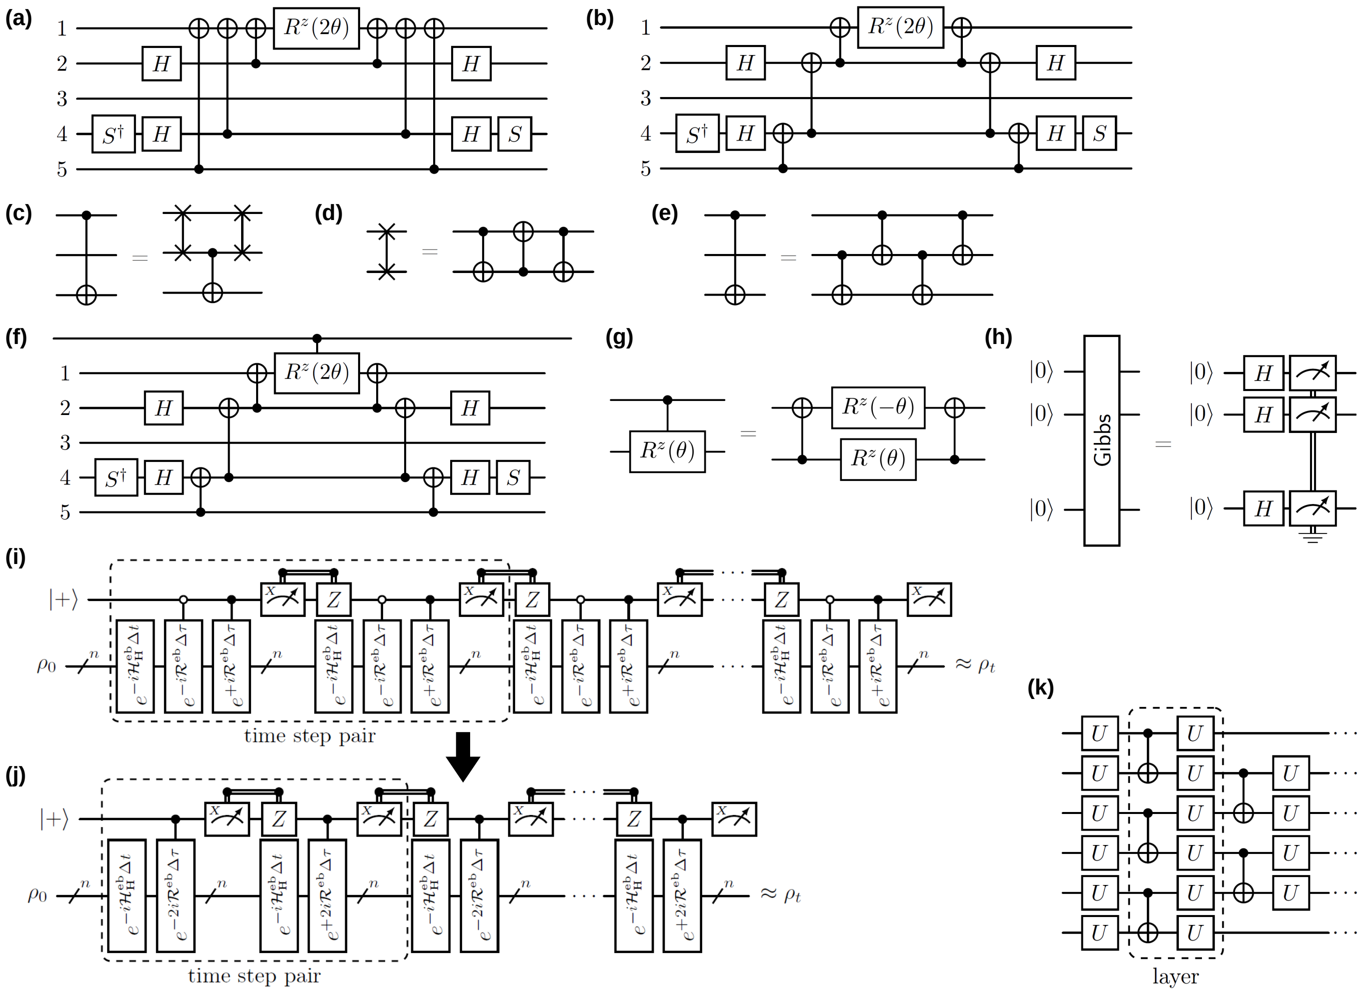


Supplementary Figure S1. **Detailed quantum simulation circuit structures and components**. **(a)** Naïve implementation of an exponentiated Pauli string $e^{-i\theta\sigma}$, also referred to as a multi-qubit Pauli rotation, comprising single-qubit Clifford basis changes and an entangler built from CX gates sandwiching a single $R^z$ rotation, as described in Supplementary Note 2 A. The Pauli string illustrated here is $\sigma = \sigma_1^z \sigma_2^x \mathbb{I}_3 \sigma_4^y \sigma_5^z$. **(b)** Alternative implementation of the same multi-qubit Pauli rotation as in (a) but with the entangler constructed via CX ladders, which reduces the number of long-range CXs and is more suitable for hardware. **(c)** A non-nearest neighbor CX gate can be reduced to a nearest-neighbor one through insertion of SWAP gates. Longer-range CXs can be decomposed in the same manner recursively. **(d)** A SWAP gate decomposes into 3 CX gates. **(e)** Bridge gate construction for non-nearest neighbor CX gates, which is more efficient in CX gate count than the SWAP insertion approach. Likewise, longer-range CXs can be decomposed recursively. **(f)** A coherently controlled $e^{-i\theta\sigma}$ amounts to inserting a control on the central single-qubit $R^z$ rotation. **(g)** A controlled-$R^z$ gate decomposes into CX gates and 2 single-qubit $R^z$ rotations. **(h)** The $\infty$-temperature Gibbs state (*i.e.* maximally mixed state) can be prepared by mid-circuit measuring qubits prepared in the $|+\rangle$ product state and discarding the measurement outcomes. **(i)** Our architecture of time-evolution circuits for non-Hermitian Hamiltonians as described in the main text, Methods and in Supplementary Note 2 B, comprising time steps of $\mathcal{M}_{\mathrm{H}}$ and $\mathcal{M}_{\mathrm{A}}$ maps approximating evolution by the Hermitian and anti-Hermitian parts of the Hamiltonian respectively. $\mathcal{M}_{\mathrm{A}}$ is achieved through a linear combination of unitaries (LCU) construction, superposing forward and backward time-evolution. A pair of adjacent time steps is highlighted. **(j)** Merging of a pair of time steps as described in Supplementary Note 2 B b, which halves the circuit depth of $\mathcal{M}_{\mathrm{A}}$ by removing a LCU term from each of the time steps. **(k)** Ansatz for circuit recompilation, comprising an interleaved brickwork pattern of CX gates and $U(2)$ single-qubit rotations. The angles of the single-qubit rotations are treated as variational parameters.

## Supplementary Note 3: Further details on error suppression and mitigation methods

### A. Zero-noise extrapolation with physicality constraints

As described in Methods, we employed zero-noise extrapolation (ZNE) as an error mitigation technique [17–21] to reduce the effects of hardware noise (*e.g.* gate errors and decoherence) on our experiment results. To review, we performed repetitions of each experiment circuit at noise amplification factors $1 = \lambda_1 < \lambda_2 < \ldots < \lambda_r$, where $\lambda = 1$ corresponds to the unmodified experiment. We assumed an affine relation between $\langle O_k^{(\lambda)} \rangle$ and $\lambda$,

$$\langle O_k^{(\lambda)} \rangle \approx m_k \lambda + c_k, \tag{S3.1}$$

where $\{O_k\}_k$ are the measured observables on the circuit, and $\{m_k\}_k$ and $\{c_k\}_k$ are gradients and zero-noise intercepts respectively. Thus, with $\langle O_k^{(\lambda)} \rangle$ data measured on hardware at $\lambda_1, \ldots, \lambda_r$, we perform the least-squares regression

$$(\mathbf{m}^*, \mathbf{c}^*) = \underset{\mathbf{m},\mathbf{c}}{\operatorname{argmin}} \sum_k \sum_{\gamma=1}^{r} \left( m_k \lambda_\gamma + c_k - \left\langle O_k^{(\lambda_\gamma)} \right\rangle \right)^2, \tag{S3.2}$$

to find best-fit gradients $\mathbf{m}^*$ and intercepts $\mathbf{c}^*$, as also expressed in Eq. (27) of Methods. On top of this standard ZNE procedure, we imposed physicality constraints on the regression to ensure that our mitigated expectation values (and the regression itself) are physically meaningful. We elaborate on these constraints below.

- *Experiments in p-particle Fock sector measuring site-resolved occupancies, that is,* $\{O_k\}_k = \{n_{x\ell}\}_{x\ell}$. This includes, for example, the experiments shown in Figures 2, 3, 5, 6 of the main text, and Supplementary Figures S2 to S6. For these, we invoked number conservation, which dictates that the number of particles in the system when measured must be $p$—otherwise an unphysical violation of the number-conserving symmetry of the system has taken place—and hardcore bosonic statistics of the particles in our system, which forbid double occupancy and thus constrains $0 \le \langle n_{x\ell} \rangle \le 1$ for all sites. Explicitly, we require

$$\sum_k \left\langle O_k^{(\lambda)} \right\rangle = p \quad \wedge \quad 0 \le \left\langle O_k^{(\lambda)} \right\rangle \le 1, \tag{S3.3}$$

  at all noise factors $0 \le \lambda \le \lambda_r$, even at intermediary levels not directly measured on hardware but implied by the regression. On the affine relation of Eq. (S3.1), this translates into regression constraints

$$\sum_k m_k = 0 \quad \wedge \quad \sum_k c_k = 1 \quad \wedge \quad \mathbf{0} \le \mathbf{c} \le \mathbf{1} \quad \wedge \quad \mathbf{0} \le \mathbf{m}\lambda_r + \mathbf{c} \le \mathbf{1}. \tag{S3.4}$$

- *Experiments measuring the imaginary energy in the p-particle sector, that is* $\{O_k\}_k = \{\mathcal{H}_{\mathrm{A}}^{\mathrm{eb}}\}$. This includes, for example, the experiments shown in Figure 4 of the main text. For these we invoked the purely lossy character of $\mathcal{H}^{\mathrm{eb}}$, that is, that $\mathcal{H}_{\mathrm{A}}^{\mathrm{eb}}$ is positive semi-definite, which dictates that $\langle \mathcal{H}_{\mathrm{A}}^{\mathrm{eb}} \rangle \le 0$. Furthermore, as there are $p$ conserved particles in the quantum system and the smallest eigenenergy of $\mathcal{H}_{\mathrm{A}}^{\mathrm{eb}}$ is $-\gamma$, by the variational principle the imaginary energy of any quantum state must satisfy $-p\gamma \le \langle \mathcal{H}_{\mathrm{A}}^{\mathrm{eb}} \rangle$. These physicality bounds should hold at all noise factors $0 \le \lambda \le \lambda_r$, just as in the case above. On the affine relation of Eq. (S3.1), this translates into regression constraints

$$-p\gamma \le c \le 0 \quad \wedge \quad -p\gamma \le m\lambda_r + c \le 0, \tag{S3.5}$$

  where we have dropped the vector notations for $\mathbf{m}, \mathbf{c}$ as there is only a single measured observable in this context.

We remark that the affine relation in Eq. (S3.1) is not a unique choice and is effectively a linear approximation—the exact variation of $\langle O_k^{(\lambda)} \rangle$ with noise amplification factor $\lambda$ is in reality an unknown function of the observables, circuit structure, and hardware error characteristics. Prior studies have examined [17–21] other ansatzes, the most common choices other than affine being a quadratic or exponential variation of $\langle O_k^{(\lambda)} \rangle$ with $\lambda$. As our circuits are non-Clifford and the hardware noise experienced in experiments is not generally simply a depolarizing channel, there is no strong theoretical justification for any of these other ansatzes, and we did not employ them for simplicity in our work. An additional theoretical challenge is also that these other ansatzes do not, strictly speaking, allow certain physical constraints to hold, unlike the affine relation. For example, as these other regression ansatzes are non-linear, they generally do not support number conservation, as in $\sum_k \langle O_k^{(\lambda)} \rangle = p$ in Eq. (S3.3), across all noise noise amplification factors $0 \le \lambda \le \lambda_r$. Therefore the physical soundness of the regression result using these other ansatzes, in our context, would be unclear.

### *a. Amplifying noise through local gate folding*

To artificially amplify noise to factors $\lambda > 1$, we employed randomized local gate folding (see *e.g.* Ref. [20]), which probabilistically replaces each gate $G$ in the circuit by $GG^\dagger G$, as described in Methods. Amplifying the number of gates in the circuit directly amplifies accumulated noise from gate errors, but also increases circuit depth and thereby amplifies, for example, thermal relaxation and dephasing noise (*i.e.* background decoherence). We comment that we perform folding such that the total number of 1- and 2-qubit gates in the circuit is each increased by factor $\lambda$. Merely targeting an increase in the total number of gates in the circuit, irrespective of their type, by $\lambda$ is insufficient. This is because the error rates of 1- and 2-qubit gates typically differ massively on hardware—indeed, by at least an order of magnitude on the devices used in our experiments—so amplifying the total number of gates by $\lambda$ without maintaining balance between the number of 1- and 2-qubit gates does not ensure that circuit noise is amplified by $\lambda$.

### *b. Randomizing coherent errors through Pauli twirling*

Lastly, we comment on the usage of randomized Pauli twirling [18, 22, 23] in producing circuits for ZNE. As described in Methods, for each experiment circuit at each $\lambda$, we produced a set of randomized gate-folded circuits and applied randomized Pauli twirling on those circuits. These circuits were executed on hardware and their results averaged, to produce the $\langle O_k^{(\lambda)} \rangle$ data for regression. The advantage of applying randomized Pauli twirling is that 2-qubit error processes on the circuits, which are the dominant source of noise, are diagonalized into incoherent stochastic (Pauli) noise channels [18, 22, 23], which can be straightforwardly averaged over (across circuit shots and realizations) in experiments. This results in more consistent trends of $\langle O_k^{(\lambda)} \rangle$ against $\lambda$, which ZNE relies upon. Without this conversion of noise processes, consistency of $\langle O_k^{(\lambda)} \rangle$ trends is less certain. For example, the coherent composition of coherent error channels (*e.g.* unitary errors arising from gate angle mis-calibration) means that the measured $\langle O_k^{(\lambda)} \rangle$ on a circuit instance can be sensitive to the exact gates selected to be folded.

## Supplementary Note 4: Additional Results

### A. Additional experiment results on the canonical edge burst

In Figure 2 and surrounding discussion of the main text, we described hardware results on an $N = 8$-unit cell quantum ladder in the edge burst and trivial regimes. In Supplementary Figure S2 below, we present an analogous breakdown of results on the same quantum ladder (*i.e.* the same Hamiltonian $\mathcal{H}^{\mathrm{eb}}$) but with different initial particle localizations, here at $x_0 = 4$ instead of $x_0 = 6$ in the main text. Identical to the experiments of Figure 2, we employed trotterization for our quantum simulation circuits without further compression (*e.g.* recompilation) before execution on hardware. The observations and conclusions are qualitatively identical to those in the main text. The real-space signature of the edge burst, a spike in final escape probability $\mathcal{P}_x$ at the $x = 1$ boundary, is clearly observed in the edge burst regime; in contrast in the trivial regime no boundary increase in $\mathcal{P}_x$ appears. Likewise, we observe our error mitigation strategies of zero-noise extrapolation (ZNE) and readout error mitigation (RO) to be of considerable benefit to data quality.

We additionally show a breakdown of experiment results on a smaller $N = 4$ quantum ladder in Supplementary Figure S3, employing likewise trotterization in the quantum simulation methodology. Here, we display a complete dataset of the measured site-resolved occupancy densities $\langle n_{x\ell} \rangle_{\rho_t}$ for all unit cells $x \in [4]$ on the ladder and sublattices $\ell \in \{a, b\}$. The observations are qualitatively similar to those before, namely a spike in $\mathcal{P}_x$ at the $x = 1$ boundary in the edge burst regime and an absence of this signature in the trivial regime.

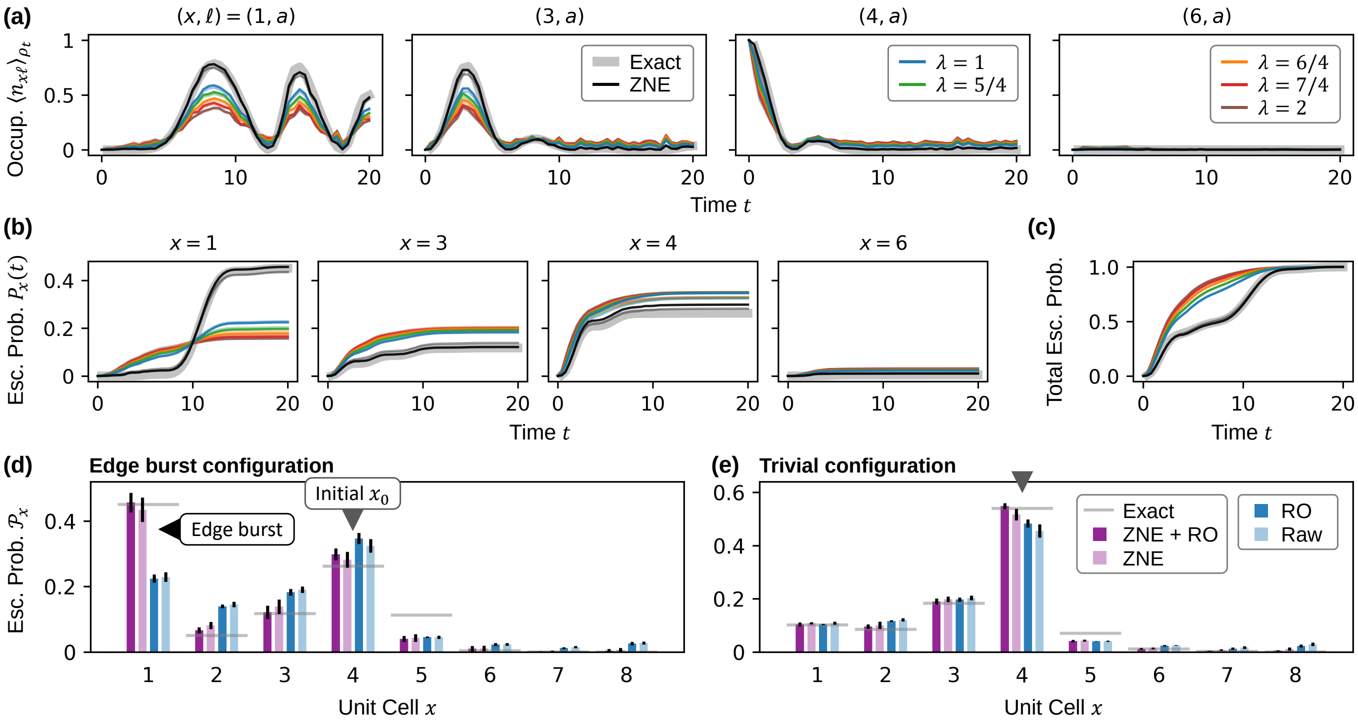


Supplementary Figure S2. **Canonical edge burst on $N = 8$ quantum ladder with different initial particle localization.** **(a)** Site-resolved occupancy densities after normalized time-evolution on a 8-unit cell quantum ladder, comparing data measured on quantum hardware at various noise amplification factors $\lambda$, after post-processing with zero-noise extrapolation (ZNE), and exact numerics. Solid thin lines are with readout error mitigation (RO) applied; translucent thin lines behind are without. To avoid clutter, only the $a$ sublattice of unit cells $x \in \{1, 3, 4, 6\}$ are shown. **(b)** Unit-cell-resolved escape probabilities $P_x(t)$ obtained from the data in (a). Time-integration of the occupancy densities first recovers proper wavefunction norm, and a second time-integration produces $P_x(t)$. **(c)** Total escape probability $P(t)$ summed over all unit cells, which approaches unity as time progresses. **(d)** Final unit-cell-resolved escape probabilities $\mathcal{P}_x$ in the long-time limit. Data obtained on quantum hardware with and without ZNE and RO, and from exact numerics, are shown. In a parameter regime supporting the edge burst, anomalously high escape probability on the $x = 1$ edge of the ladder is detected; whereas in the trivial regime escape probability is concentrated only near the initial location of the particle (at $x_0 = 4$). Error bars are standard deviations across 8 experiment runs. See Supplementary Tables S1 and S2 for Hamiltonian parameter values and superconducting quantum devices used. The experiments shown here complement Figure 2 of the main text, which reports results on the same quantum ladder but with different initial particle locations (there $x_0 = 6$).

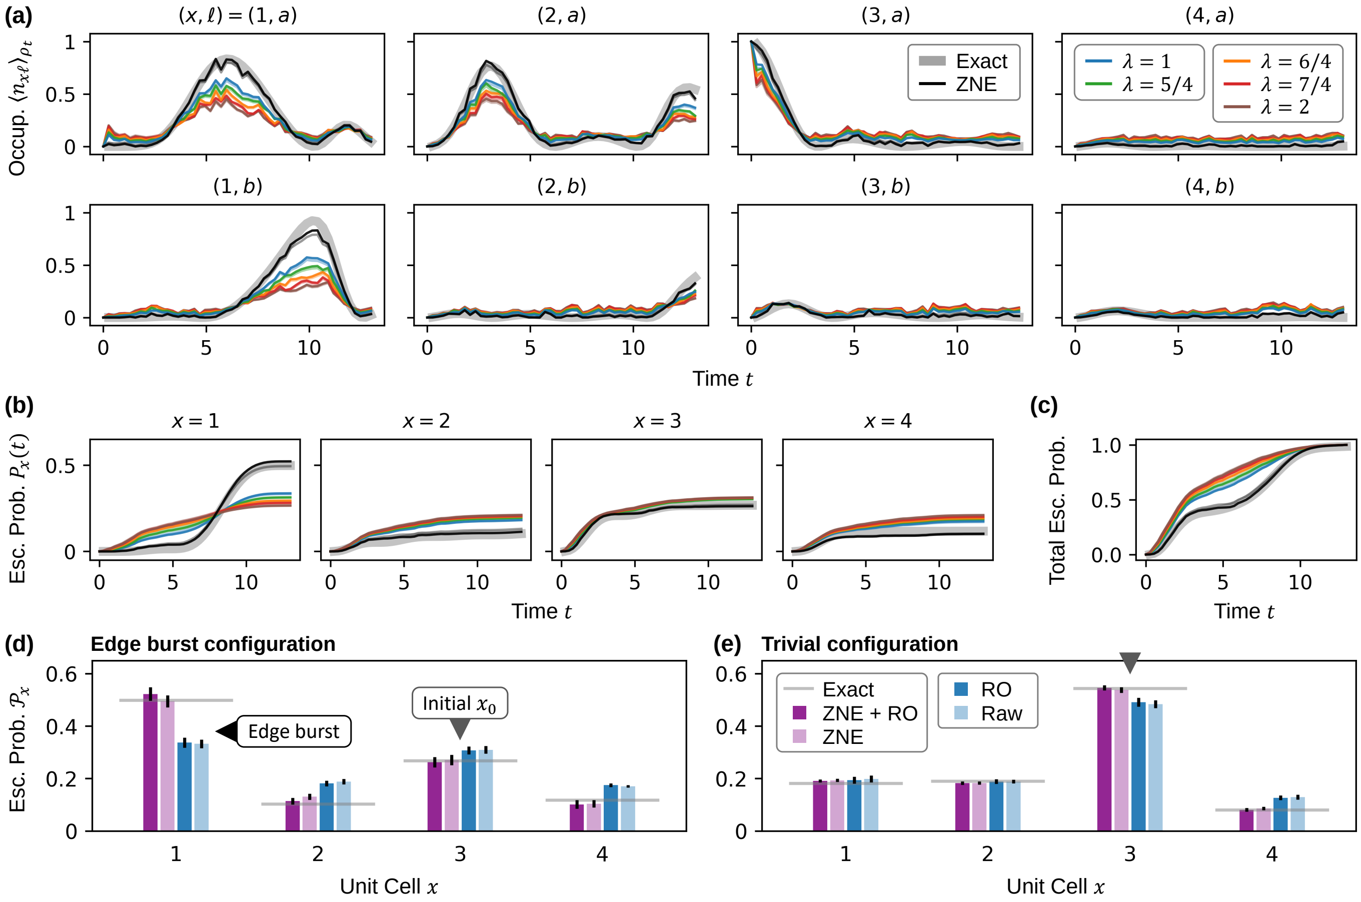


Supplementary Figure S3. **Canonical edge burst on a smaller $N = 4$ quantum ladder.** **(a)** Site-resolved occupancy densities after normalized time-evolution on a 4-unit cell quantum ladder, comparing data measured on quantum hardware at various noise amplification factors $\lambda$, after post-processing with zero-noise extrapolation (ZNE), and exact numerics. Solid thin lines are with readout error mitigation (RO) applied; translucent thin lines behind are without. **(b)** Unit-cell-resolved escape probabilities $P_x(t)$ obtained from the data in (a). Time-integration of the occupancy densities first recovers proper wavefunction norm, and a second time-integration produces $P_x(t)$. **(c)** Total escape probability $P(t)$ summed over all unit cells, which approaches unity as time progresses. **(d)** Final unit-cell-resolved escape probabilities $\mathcal{P}_x$ in the long-time limit. Data obtained on quantum hardware with and without ZNE and RO, and from exact numerics, are shown. In a parameter regime supporting the edge burst, anomalously high escape probability on the $x = 1$ edge of the ladder is detected; whereas in the trivial regime escape probability is concentrated only near the initial location of the particle (at $x_0 = 3$). Error bars are standard deviations across 8 experiment runs. See Supplementary Tables S1 and S2 for Hamiltonian parameter values and superconducting quantum devices used. The experiments shown here complement Figure 2 of the main text and Supplementary Figure S2, which report results on a larger $N = 8$ quantum ladder.

### B. Spatially extended edge bursts with multiple interacting particles

In Figure 5 and surrounding discussion of the main text, we described the possibility of obtaining spatially extended edge bursts spanning multiple unit cells, in contrast to the canonical single-particle edge burst that occurs on a single unit cell, and which exhibit spatial ordering, when multiple interacting particles are present on the quantum ladder. There, we began by examining experiments with two interacting particles. Figures 5a, 5c and 5d reported hardware results in the edge burst without ordering and with $\mathbb{Z}_2$ and $\mathbb{Z}_3$ ordering respectively, where the occurrence of the edge burst is clearly observed, while Figure 5b reported results without ordering in the trivial regime. As validation that this is indeed an edge burst phenomenon, the spatially ordered edge bursts should vanish in the trivial regime. We verify this in Supplementary Figure S4, which presents hardware results directly analogous to Figures 5c and 5d of the main text but in the trivial regime.

Additionally, as also discussed in the main text, the same phenomenon of spatially extended and ordered edge bursts can be observed with larger numbers of interacting particles. With $p$ particles, it is generically possible to obtain edge bursts extended over $p$ unit cells from the boundary. Here, we report hardware results with three interacting particles in Supplementary Figure S5. A spatially extended edge burst is seen in Supplementary Figure S5a, and edge bursts with $\mathbb{Z}_2$ and $\mathbb{Z}_3$ ordering are observed in Supplementary Figure S5c and Supplementary Figure S5e respectively. Supplementary Figures S5b, S5d and S5f show results in the trivial regime, in which no edge burst arises.

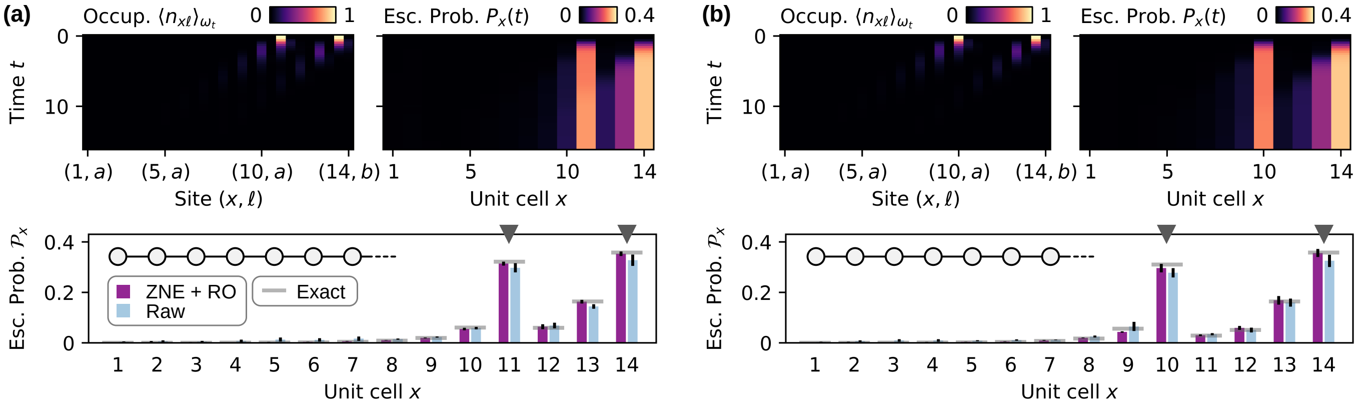


Supplementary Figure S4. **Additional results with two interacting particles.** **(a)** Site-resolved occupancy densities and unit-cell-resolved escape probabilities $P_x(t)$ measured on a 14-unit cell quantum ladder in the trivial regime hosting two interacting particles. The quantum ladder has density-density interactions $U_r > 0$ switched on for $r \leq 3$. Final escape probabilities $\mathcal{P}_x$ obtained on hardware with and without zero-noise extrapolation (ZNE) and readout error mitigation (RO), and exact numerics, are shown. Gray arrows denote the initial localization of the particles. **(b)** Same as (a) but with longer-ranged interactions, $U_r > 0$ switched on for $r \leq 5$, and with correspondingly larger separation in initial localization of the particles. Error bars are standard deviations across 10 experiment runs. See Supplementary Tables S1 and S2 for Hamiltonian parameter values and superconducting quantum devices used. No edge burst is observed in both (a) and (b). Panels (a) and (b) complement Figures 5c and 5d in the main text respectively, which show results in the edge burst regime.

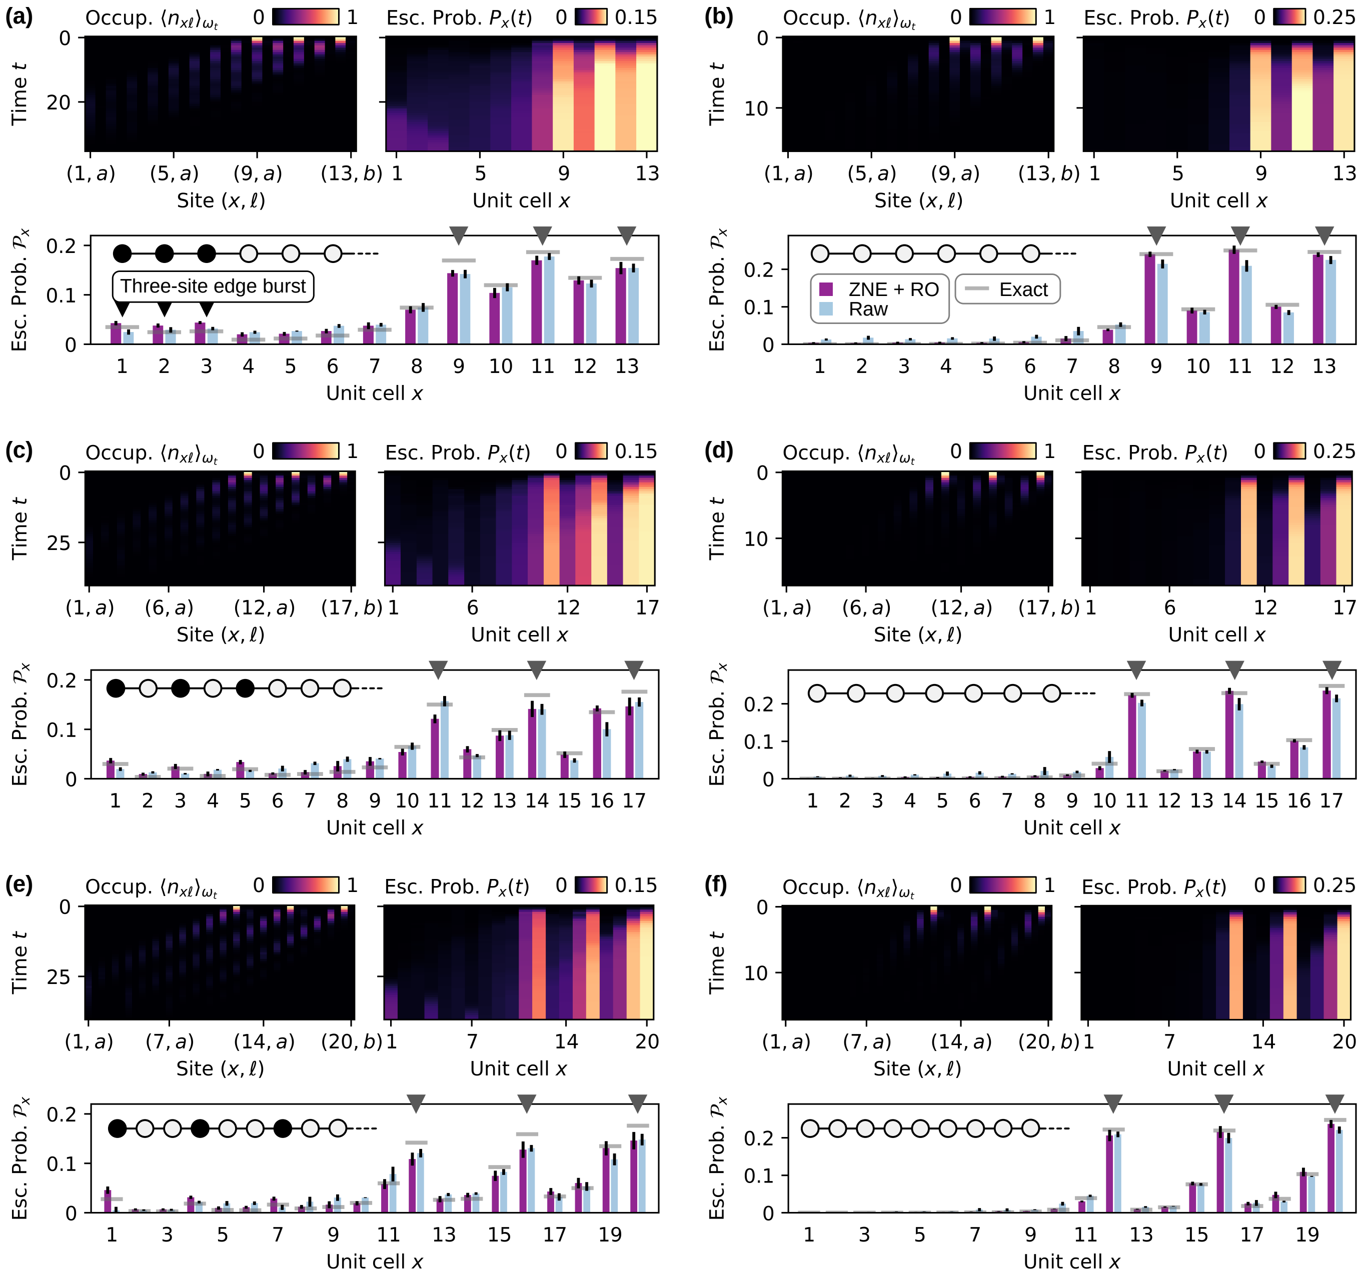


Supplementary Figure S5. **Spatially extended and ordered edge bursts with three interacting particles. (a)** Site-resolved occupancy densities and unit-cell-resolved escape probabilities $P_x(t)$ measured on a 13-unit cell quantum ladder in the edge burst regime hosting three interacting particles. The quantum ladder has density-density interactions $U_r > 0$ switched on for $r = 1$. Final escape probabilities $\mathcal{P}_x$ obtained on hardware with and without zero-noise extrapolation (ZNE) and readout error mitigation (RO), and exact numerics, are shown. Gray arrows denote the initial localization of the particles. **(b)** Same as (a) but in the trivial regime. **(c)**, **(e)** Occupancy densities, escape probabilities $P_x(t)$, and final escape probability $\mathcal{P}_x$ on (c) a 17-unit cell ladder with interactions $U_r > 0$ switched on for $r \leq 3$, and a 20-unit cell ladder with interactions $U_r > 0$ for $r \leq 5$, in the edge burst regime. **(d)**, **(f)** Same as (c) and (e) respectively but in the trivial regime. Spatially extended edge bursts are observed in (a), (c), (e), with $\mathbb{Z}_2$ and $\mathbb{Z}_3$ ordering in (c) and (e) respectively. The spatial patterns of edge bursts on unit cells are illustrated as black shading in the cartoon insets. Error bars are standard deviations across 10 experiment runs. See Supplementary Tables S1 and S2 for Hamiltonian parameter values and superconducting quantum devices used. The experiments shown here extend Figure 5 of the main text and Supplementary Figure S4 which were with two interacting particles.

### C. Alternative recovery of quantum state norm from algorithm success probability

To review, recall that time-evolution by a non-Hermitian Hamiltonian $\mathcal{H}$ is non-unitary, and the norm of a quantum state is not generically preserved during time-evolution. That is, examining the physical time-evolved state $\omega_t = e^{-i\mathcal{H}t}\omega_0 e^{+i\mathcal{H}^\dagger t}$ from an initial state $\omega_0$, generically $\mathrm{tr}\,\omega_t \neq \mathrm{tr}\,\omega_0 = 1$. As mentioned in the main text and Methods, to realize time-evolution on a quantum platform in experiments, we perform normalized time-evolution, $\rho_t = \mathcal{N}[e^{-i\mathcal{H}t}\rho_0 e^{+i\mathcal{H}^\dagger t}]$, where $\rho_0 = \omega_0$. The normalized state $\rho_t$ is related to $\omega_t$ by a rescaling, $\omega_t = A_t^2 \rho_t$. Accordingly, by measuring any observable $O$ on the normalized time-evolved state $\rho_t$ in the experiment, we can rescale the measurement results to be on $\omega_t$, by the relation $\langle O \rangle_{\omega_t} = A_t^2 \langle O \rangle_{\rho_t}$.

The method employed to recover $A_t$ in all our reported experiments is through a double time-integration of measured occupancy density $\langle n_{x\ell} \rangle_{\rho_t}$ data, as was described in detail in the main text and Methods. But as described in Methods, there is an alternative method available. Namely, the quantum simulation algorithm for normalized time-evolution succeeds precisely with a probability $S_t$ directly related to the norm of the time-evolved quantum state. Provided $\mathrm{tr}\,\omega_0 = \mathrm{tr}\,\rho_0 = 1$ initially, $A_t^2 \approx S_t$ up to suppressible approximation errors in the time-evolution algorithm and circuit construction. Thus $S_t$ measured in experiments allow recovery of $A_t^2$, to then serve the same role in enabling estimation of observable expectation values $\langle O \rangle_{\omega_t}$.

In Supplementary Figure S6a, we show a concrete comparison between the two methods. We examine the same experiment as in Figure 5c of the main text, with two interacting particles on the quantum ladder producing a spatially extended edge burst with $\mathbb{Z}_2$ ordering. We report the cell-resolved final escape probabilities $\mathcal{P}_x$ obtained via the observed success rate of the time-evolution algorithm (denoted "Anc." in the figure), and for ease of comparison, include also $\mathcal{P}_x$ obtained through the time-integration method (denoted "Int.") previously shown in Figure 5c. We show also a comparison of the total escape probability $P(t)$ summed over all unit cells, obtained through the success rate and time-integration methods. In Supplementary Figure S6b we present analogous data but in the trivial regime.

Our general observation in experiments is that both methods of recovering the quantum state norm give very similar results after error mitigation. Indeed here, in the example shown in Supplementary Figure S6, the $\mathcal{P}_x$ spatial profiles obtained from the two methods exhibit a quantitative match within error bars. The $P(t)$ time profiles are also similar; the small differences detectable in Supplementary Figure S6 are largely inconsequential to the escape probabilities $P_x(t)$ and $\mathcal{P}_x$.

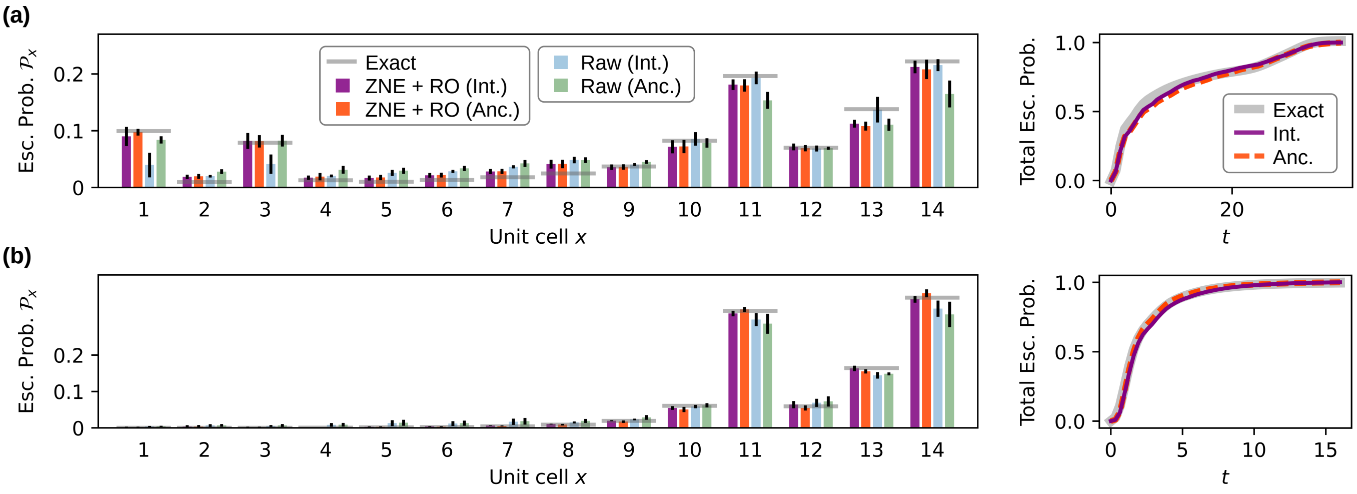


Supplementary Figure S6. **Example comparison between quantum state norm recovery methods. (a)** Final cell-resolved escape probabilities $\mathcal{P}_x$ obtained on hardware with and without zero-noise extrapolation (ZNE) and readout error mitigation (RO), and exact numerics, shown on the left. Total escape probability $P(t)$ summed over all unit cells versus time $t$, shown on the right. **(b)** Analogous experiment data but in the trivial regime. Data denoted "Int." were obtained via double time-integration of measured site-resolved occupancy densities for quantum state norm recovery, a method described in the main text and Methods, and were previously shown in Figure 5c. Data denoted "Anc." were obtained by inferring quantum state norm from algorithm success rate. Error bars are standard deviations across 10 experiment runs. See Supplementary Tables S2 and S3 for Hamiltonian parameter values and superconducting quantum devices used.

[1] W.-T. Xue, Y.-M. Hu, F. Song, and Z. Wang, Non-Hermitian edge burst, Phys. Rev. Lett. **128**, 120401 (2022).
[2] P. Wen, J. Pi, and G.-L. Long, Investigation of a non-Hermitian edge burst with time-dependent perturbation theory, Phys. Rev. A **109**, 022236 (2024).
[3] S. Yao and Z. Wang, Edge states and topological invariants of non-Hermitian systems, Phys. Rev. Lett. **121**, 086803 (2018).
[4] M. A. Nielsen and I. L. Chuang, *Quantum computation and quantum information* (Cambridge university press, 2010).
[5] T. Itoko, R. Raymond, T. Imamichi, and A. Matsuo, Optimization of quantum circuit mapping using gate transformation and commutation, Integration **70**, 43 (2020).
[6] J. Welch, A. Bocharov, and K. M. Svore, Efficient approximation of diagonal unitaries over the Clifford+T basis (2015), arXiv:1412.5608 [quant-ph].
[7] M. Ezawa, Systematic construction of square-root topological insulators and superconductors, Phys. Rev. Res. **2**, 033397 (2020).
[8] A. M. Marques, L. Madail, and R. G. Dias, One-dimensional $2^n$-root topological insulators and superconductors, Phys. Rev. B **103**, 235425 (2021).
[9] M. Kremer, I. Petrides, E. Meyer, M. Heinrich, O. Zilberberg, and A. Szameit, A square-root topological insulator with non-quantized indices realized with photonic Aharonov-Bohm cages, Nat. Commun. **11**, 907 (2020).
[10] H. Wu, G. Wei, Z. Liu, and J.-J. Xiao, Square-root topological state of coupled plasmonic nanoparticles in a decorated Su–Schrieffer–Heeger lattice, Opt. Lett. **46**, 4256 (2021).
[11] W. Deng, T. Chen, and X. Zhang, $n$th power root topological phases in Hermitian and non-Hermitian systems, Phys. Rev. Res. **4**, 033109 (2022).
[12] L. Song, H. Yang, Y. Cao, and P. Yan, Square-root higher-order Weyl semimetals, Nat. Commun. **13**, 5601 (2022).
[13] A. M. Marques and R. G. Dias, $2^n$-root weak, chern, and higher-order topological insulators, and $2^n$-root topological semimetals, Phys. Rev. B **104**, 165410 (2021).
[14] Z. Lin, S. Ke, X. Zhu, and X. Li, Square-root non-Bloch topological insulators in non-Hermitian ring resonators, Opt. Express **29**, 8462 (2021).
[15] S. Guo, G. Pan, J. Huang, R. Huang, F. Zhuang, S. Su, Z. Lin, W. Qiu, and Q. Kan, Realization of the square-root higher-order topology in decorated Su–Schrieffer–Heeger electric circuits, Appl. Phys. Lett. **123**, 043102 (2023).
[16] Z.-G. Geng, Y.-X. Shen, Z. Xiong, L. Duan, Z. Chen, and X.-F. Zhu, Quartic-root higher-order topological insulators on decorated three-dimensional sonic crystals, APL Mater. **12**, 021108 (2024).
[17] Y. Kim, A. Eddins, S. Anand, K. X. Wei, E. Van Den Berg, S. Rosenblatt, H. Nayfeh, Y. Wu, M. Zaletel, K. Temme, *et al.*, Evidence for the utility of quantum computing before fault tolerance, Nature **618**, 500 (2023).
[18] Y. Kim, C. J. Wood, T. J. Yoder, S. T. Merkel, J. M. Gambetta, K. Temme, and A. Kandala, Scalable error mitigation for noisy quantum circuits produces competitive expectation values, Nat. Phys. **19**, 752 (2023).
[19] R. Majumdar, P. Rivero, F. Metz, A. Hasan, and D. S. Wang, Best practices for quantum error mitigation with digital zero-noise extrapolation, in *2023 IEEE International Conference on Quantum Computing and Engineering (QCE)*, Vol. 1 (IEEE, 2023) pp. 881–887.
[20] T. Giurgica-Tiron, Y. Hindy, R. LaRose, A. Mari, and W. J. Zeng, Digital zero noise extrapolation for quantum error mitigation, in *2020 IEEE International Conference on Quantum Computing and Engineering (QCE)* (IEEE, 2020) pp. 306–316.
[21] K. Temme, S. Bravyi, and J. M. Gambetta, Error mitigation for short-depth quantum circuits, Phys. Rev. Lett. **119**, 180509 (2017).
[22] A. Hashim, R. K. Naik, A. Morvan, J.-L. Ville, B. Mitchell, J. M. Kreikebaum, M. Davis, E. Smith, C. Iancu, K. P. O'Brien, I. Hincks, J. J. Wallman, J. Emerson, and I. Siddiqi, Randomized compiling for scalable quantum computing on a noisy superconducting quantum processor, Phys. Rev. X **11**, 041039 (2021).
[23] J. J. Wallman and J. Emerson, Noise tailoring for scalable quantum computation via randomized compiling, Phys. Rev. A **94**, 052325 (2016).
